# Supplementary material for: Machine Learning Diffusion Monte Carlo Forces
Source: arXiv:2211.07103 source file (2022-11-14)
Supplement: Supplementary file 1 [file SI.pdf]

# Supplementary Materials for "Machine Learning Diffusion Monte Carlo Forces"

Cancan Huang and Brenda M. Rubenstein*

*Department of Chemistry, Brown University, Providence, Rhode Island, 02912, USA*

E-mail: brenda_rubenstein@brown.edu

## AMPtorch Model Hyperparameter Tuning

In this section, we explain in detail the hyperparameter tuning we performed for our AMPtorch models taking $C_2$ as an example. The AMPtorch models for $H_2O$ and $CH_3Cl$ were optimzed in the same manner. The best combination of hyperparameters was selected based upon their performance on our training and test datasets when trained without forces. To understand the influence of different hyperparameters on our model, especially the models trained without forces, we selected the number of layers in our neural networks, number of nodes in each of the networks' layers, and learning rates for optimization while keeping all other hyperparameters, such as the batch size and number of training epochs, the same. Table S1 shows the hyperparameter values tuned during our optimization process.

As described in the Computational Methods section, the AMPtorch models are based on Behler-Parrinello Neural Networks, which describe each atom using its adjacent atoms and construct different subnets for each atomic species. Each subnet is a fully-connected neural network, with the

**Table S1:** Hyperparameters and hyperparameter values tested to optimize the number of layers, the number of nodes per layer, and the learning rate in our model. Layers and nodes are referred to as the subnet in BPNN discussions. Different models were built using each combination and then trained and tested on $C_2$ dataset for best performance. The number of possible hyperparameter combinations leads to 448 total different models.

| Hyperparameter | Values |
|---|---|
| **Number of layers** | 2, 3, 5, 7, 9, 12, 15, 20 |
| **Number of nodes per layer** | 2, 5, 10, 15, 20, 25, 30, 40 |
| **Learning rate** | 0.1, 0.05, 0.01, 0.005, 0.001, 0.0005, 0.0001 |
| $\alpha$ **coefficient** (only for models with forces) | 0.001, 0.01, 0.1, 1.0, 10.0, 20.0 |

same number of nodes in each layer. The loss function for the model can be written as

$$\begin{aligned} L_{energy} &= \frac{1}{N_{batch}} \sum_{i}^{N_{batch}} (E_i^{reference} - E_i^{prediction})^2 \\ L_{forces} &= \frac{1}{3N_{batch}} \sum_{i}^{N_{batch}} \sum_{k=1}^{3} (F_{i,k}^{reference} - F_{i,k}^{prediction})^2 \\ L_{total} &= \frac{1}{2}(L_{energy} + \alpha \cdot L_{forces}), \end{aligned} \tag{1}$$

where $N_{batch}$ is the number of points in each training batch and $\alpha$ is the force coefficient for the loss value, which represents the weight of the forces loss in the total loss. When the model is trained without forces, $\alpha = 0$; when the model is trained with forces, $\alpha > 0$.

We then trained different AMPtorch DFT models without forces with different hyperparameters settings. Comparing the performance of all 448 different AMPtorch DFT models without forces, we found that the AMPtorch model with a subnet that consists of 3 layers with 5 nodes in each layer trained with a learning rate of 0.001 yields the best MAE value on the $C_2$ dataset. How the energy MAE changes with each hyperparameter is presented in Figure S1.

Another important hyperparameter that needs to be considered is the force coefficient, $\alpha$, when training AMPtorch models with forces. Here, we chose the same architecture for AMPtorch DFT models with forces as we did for AMPtorch DFT models without forces. We intentionally structured our models this way to reveal the influence of adding forces to our model while eliminating the possible artificial effects induced by adding potentially irrelevant hyperparameters. The influ-

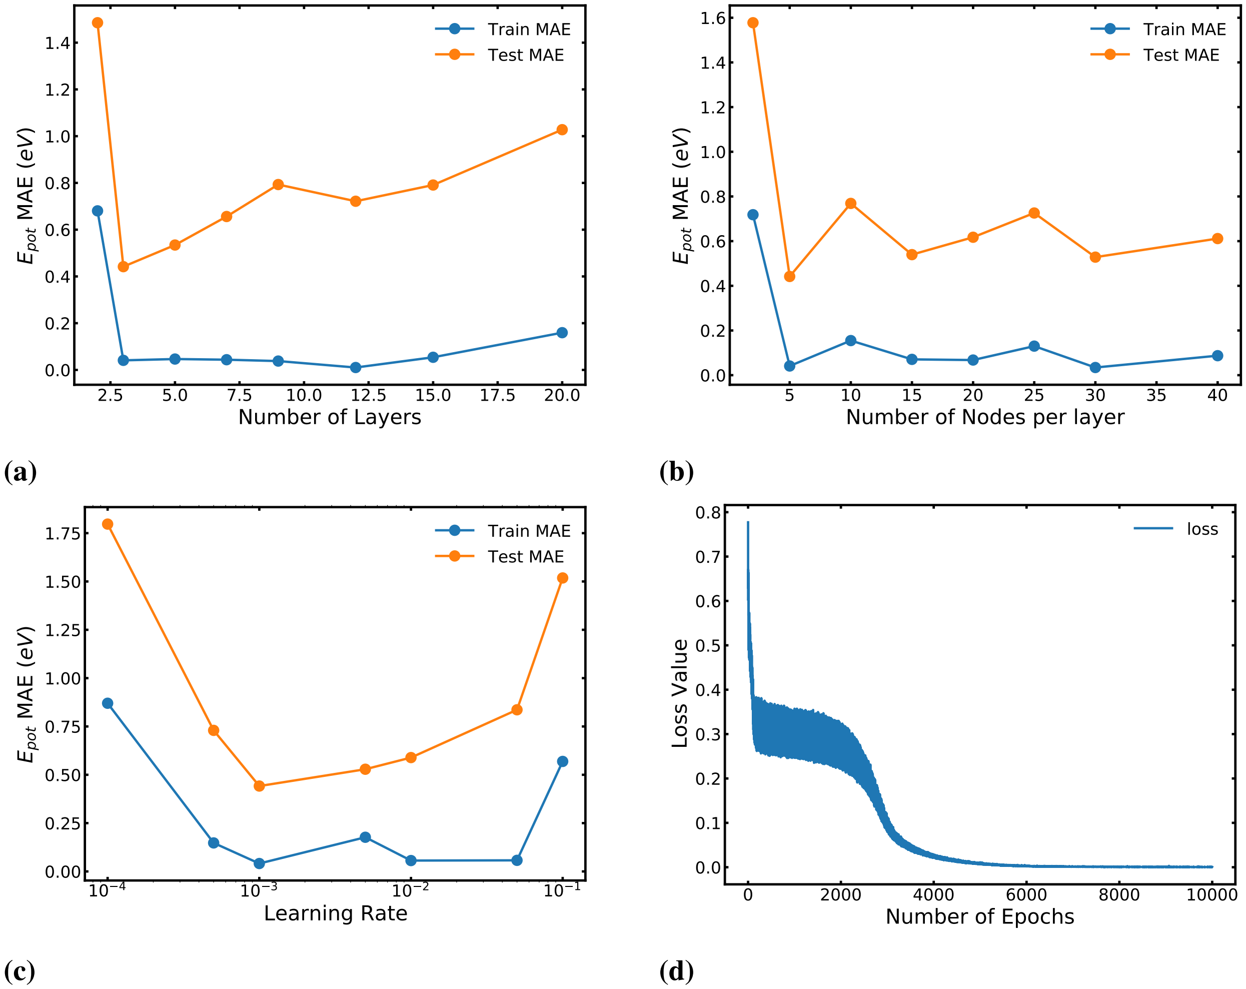


**Figure S1:** Energy MAEs on the training and test data sets for the AMPtorch DFT model without forces for $C_2$. (**a**): Energy MAE vs. number of layers holding the number of nodes per layer to 5 and the learning rate to 0.001; (**b**): Energy MAE vs. number of nodes per layer holding the number of layers to 3 and the learning rate to 0.001; (**c**): The energy MAE vs. learning rate holding the number of layers to 3 and the number of nodes per layer to 5. Based on these figures, it can be observed that the model performs optimally when it has 3 layers with 5 nodes in each layer and is trained with a learning rate of 0.001. (**d**): The loss value for the model with 3 layers and 5 nodes per layer and trained with a learning rate of 0.001. The curve flattened at the end of the training process, meaning that the model is well-converged.

ence of the force coefficient, $\alpha$, on both energy and force predictions is presented in Figure S2. We found that when $\alpha$ is 1.0, the AMPtorch model showed the best performance.

In summary, for $C_2$, the AMPtorch models consist of subnets of 3 layers with 5 nodes in each layer and were trained using a learning rate of 0.001. When these models were trained with forces, they performed best when the $\alpha$ in the loss function was 1.0. For $H_2O$ and $CH_3Cl$, the hyperparameters were also optimized using the same procedure. The best model hyperparameter combinations for each case are summarized in Table S2.

**Table S2:** Summary of optimal model hyperparameters for $C_2$, $H_2O$, and $CH_3Cl$. All of the AMPtorch models used for each case study (e.g., $C_2$, $H_2O$, $CH_3Cl$) employed the same architecture.

| Example | Number of layers | Number of nodes per layer | Learning rate | $\alpha$ coefficient |
|---|---|---|---|---|
| $C_2$ | 3 | 5 | 0.001 | 1.0 |
| $H_2O$ | 5 | 10 | 0.0001 | 0.01 |
| $CH_3Cl$ | 5 | 10 | 0.001 | 1.0 |

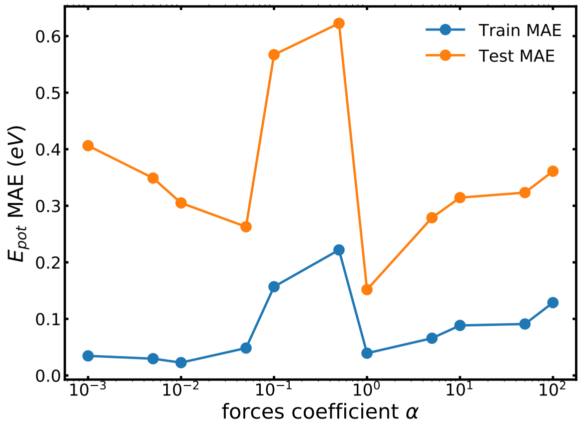


(a)

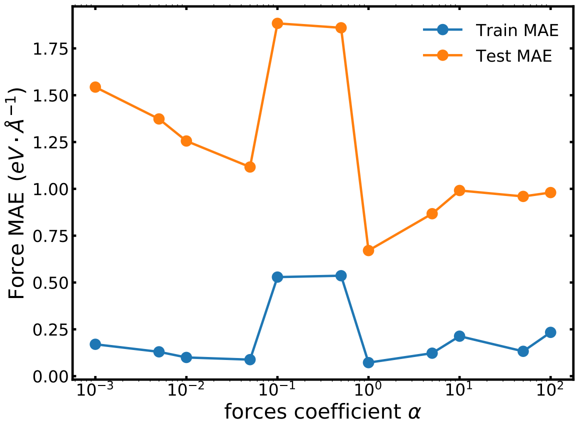


(b)

**Figure S2:** Energy and force MAEs on training and test and test datasets of $C_2$ for the AMPtorch DFT model with forces. **(a)**: Energy MAEs vs. force coefficient, $\alpha$; **(b)**: Force MAEs vs. force coefficient, $\alpha$. From the above figures, it can be observed that the training and test MAEs are lowest on energy and force predictions when the force coefficient approaches 1. Too small or too large of a force coefficient will decrease model performance.

# AMPtorch DFT Model MAEs vs. Number of Training Labels

According to previous literature, a more just way of assessing the change in the MAE with respect to the amount of energy and force training points provided is to plot the MAE with respect to the number of training labels, where each energy and each force component corresponds to one training label. In the following, we have plotted the $C_2$ Energy MAE for the AMPtorch-DFT models, with and without forces, against the number of training labels in the training dataset. For the carbon dimer, when the AMPtorch DFT model is trained without forces, only one energy label is used; when it is trained with forces, six additional force labels are used to optimize the model, bringing the total number of labels to seven. To compensate for the fact that training with forces actually uses more training labels, Figure S3 uses "number of training labels" as its x axis. We have observed that when the number of training labels is the same, the AMPtorch DFT model with forces and the AMPtorch DFT model without force show similar energy MAEs.

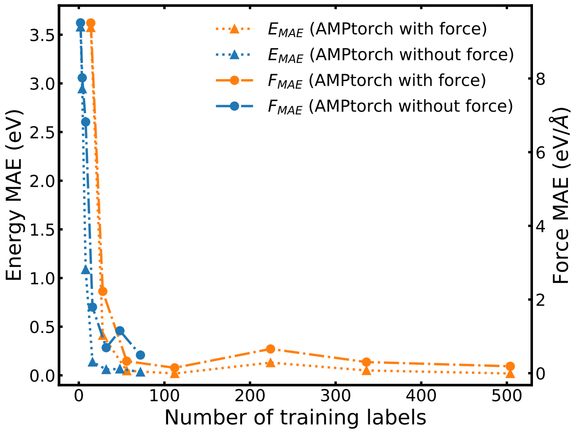


**Figure S3:** Comparison of the performance of the AMPtorch DFT (with forces) and AMPtorch DFT (without forces) models on $C_2$ trained on an increasing number training labels, where each energy and force components corresponds to a label. The performance is reported by evaluating each model on the test dataset of 48 grid-sampled points.

# AMPtorch Models Performance on the Three Example Molecules Studied in the Manuscript

Here, we report the mean-absolute-error (MAE) on the energies and forces of the three AMPtorch models on the training and test data for the three molecules studied in this manuscript, $C_2$, $H_2O$, and $CH_3Cl$. The energy MAE is calculated using the following equation

$$MAE_{\text{energy}} = \frac{1}{N}\sum_{i=1}^{N} \|E_i^{reference} - E_i^{prediction}\|. \tag{2}$$

where $N$ is the number of points in the dataset and the reference energy is the DFT energy for the AMPtorch DFT models and the DMC energy for AMPtorch DMC model.

For the force MAE, instead of calculating the MAE of the norm of the forces, we instead calculate the force MAE using the following equations

$$MAE_{\text{force}} = \frac{1}{3N}\sum_{i=1}^{N}\sum_{k=1}^{3} \|F_{i,k}^{reference} - F_{i,k}^{prediction}\|. \tag{3}$$

## $C_2$ Molecule MAE

As stated in the manuscript, training points for $C_2$ were chosen within the interval [0.7, 3.5]$\times R_0$ with different gaps between the points, where $R_0 = 1.242$ Å is $C_2$'s equilibrium bond distance. Altogether, 29 total points were included in the $C_2$ training dataset. A more dense set of points within the same interval were selected to form the test set.

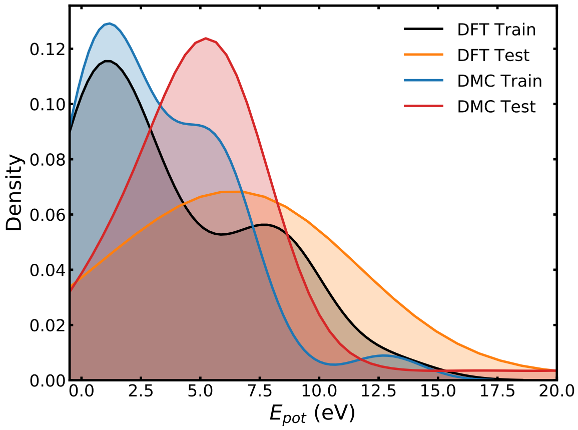


**Figure S4:** Energy distributions of the $C_2$ training and test datasets for DFT and DMC. The energy distribtions for structures in the training and test datasets are reasonably close. This can in part explain the similar MAEs values in Table S3.

Table S3 and Figures S5-S7 show the training and test results for the AMPtorch DFT (with forces), AMPtorch DFT (without forces), and AMPtorch DMC models of $C_2$. We also compared our DFT results with a Morse potential model to put the MAE errors in perspective. The Morse potential energy function has the form

$$V(r) = D_e(e^{-2a(r-r_e)} - 2e^{-a(r-r_e)}) \tag{4}$$

where $D_e$ is the potential well depth, $r_e$ is the equilibrium bond distance, and $a$ is the width of the potential well. For the Morse potential model, the Morse parameters, $D_e$, $r_e$ and $a$, were obtained by fitting to DFT energies using the *scipy.optimize.curve_fit* function. After fitting, we found that $D_e = 8.837$ eV, $r_e = 1.299$Å, and $a = 1.831$Å, which are close to the values provided in Ref. 1.

**Table S3:** MAEs on the training and test set energies and forces for $C_2$. MAEs are provided for the three models discussed in this work: the AMPtorch DFT model with forces, the AMPtorch DFT model without forces, and the AMPtorch DMC model. For the DFT calculations, the reference data are DFT energies and forces. For the AMPtorch DMC model, the reference data are DMC energies. We also fit against a Morse potential to draw a comparison between the performance of our BPNN and a simple, classical potential. For the Morse potential model, the Morse parameters, $D_e$, $r_e$ and $a$, were obtained by fitting to DFT energies using the *scipy.optimize.curve_fit* function.

| **MAE** | **AMPtorch DFT** (with forces) | **AMPtorch DFT** (without forces) | **AMPtorch DMC** | **Morse potential** (against DFT energies) |
|---|---|---|---|---|
| **Training Energies** MAE (eV/atom) | 0.0390 | 0.0410 | 0.0414 | 0.1462 |
| **Training Forces** MAE (eV/(Å atom)) | 0.0722 | 0.2007 | - | 0.2576 |
| **Test Energies** MAE (eV/atom) | 0.0406 | 0.0274 | 0.0368 | 0.3142 |
| **Test Forces** MAE (eV/(Å atom) | 0.0598 | 0.0580 | - | 0.4899 |

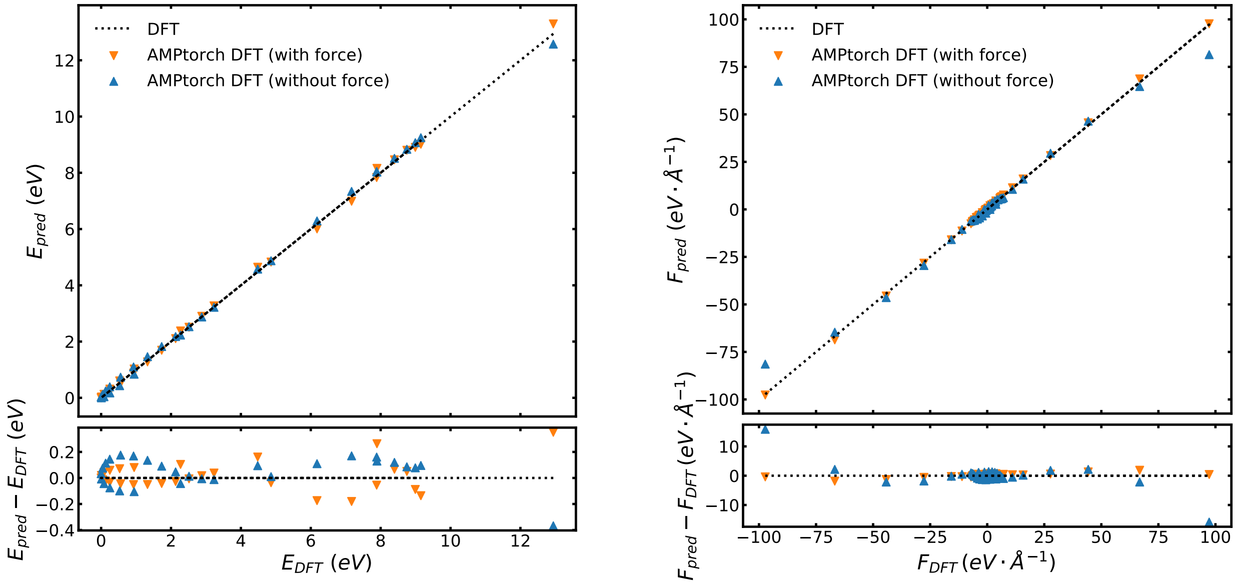


**(a)** **(b)**

**Figure S5:** (Top): Parity plots comparing the 'exact' and predicted energies (a) and forces (b) for $C_2$ obtained from different AMPtorch models for the training data. (Bottom): Differences between the predicted and 'exact' DFT energies (a) and forces (b) as a function of the DFT values. All data points are the same as those used in Figure 2 in the main text.

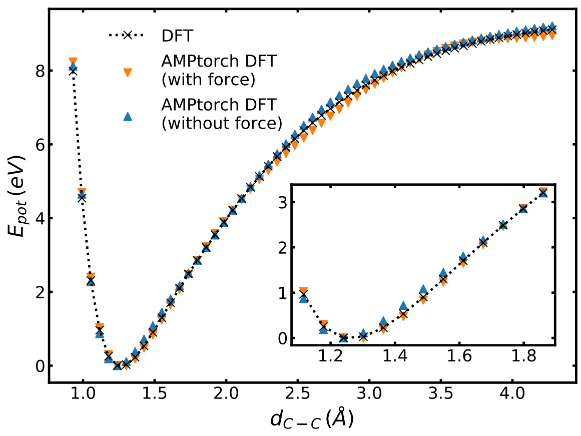


**(a)**

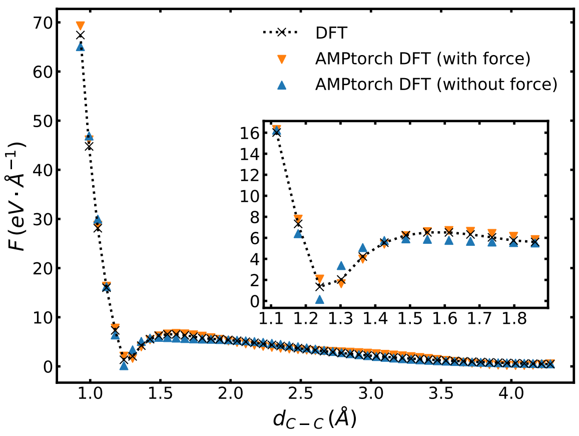


**(b)**

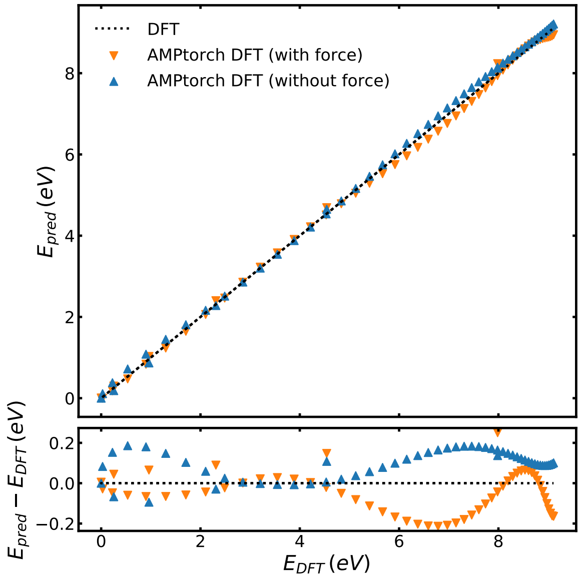


**(c)**

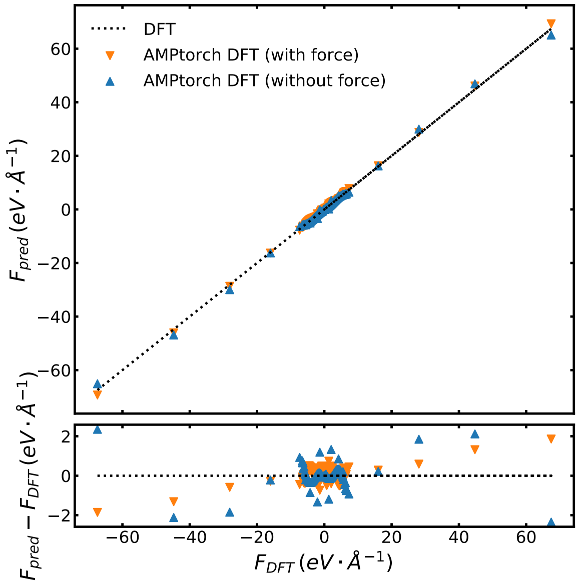


**(d)**

**Figure S6:** Comparisons between the predicted and 'exact' energies and forces for $C_2$ from DFT and the AMPtorch DFT models. (a) Potential energy vs. C-C bond distance. (b) Force vs. C-C bond distance. (c) Parity plot comparing the DFT and predicted energies as a function of the DFT energy on the test data. (d) Parity plot comparing the DFT and predicted forces as a function of the DFT energy on the test data. The test data points are evenly distributed along the C-C bond distance, ranging from 0.93 Å to 4.28 Å.

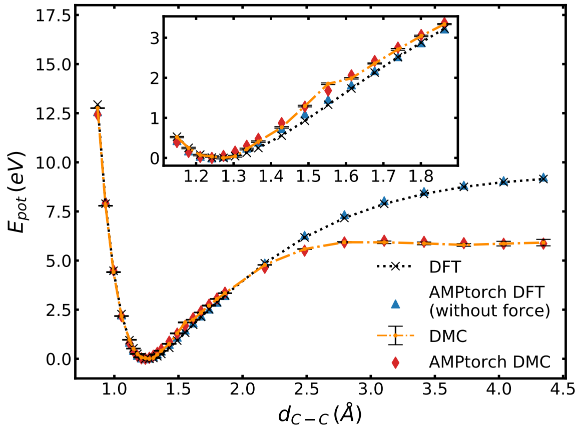


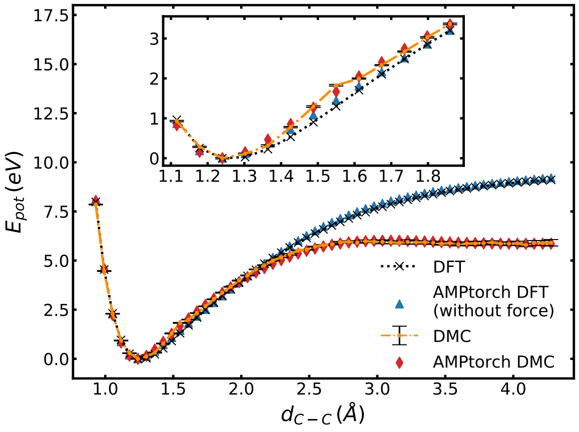


(a) (b)

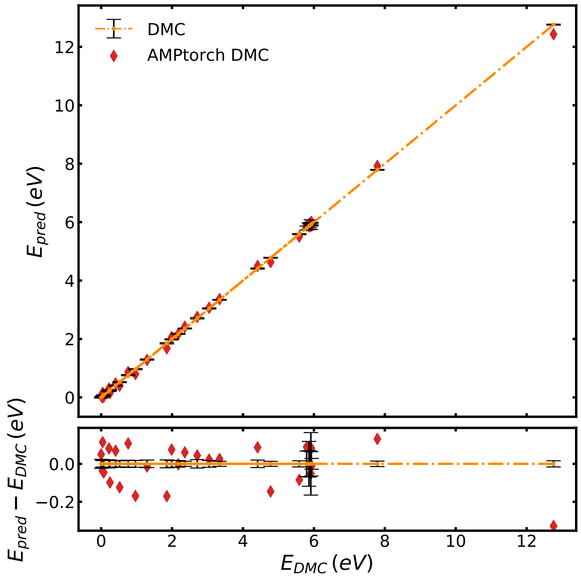


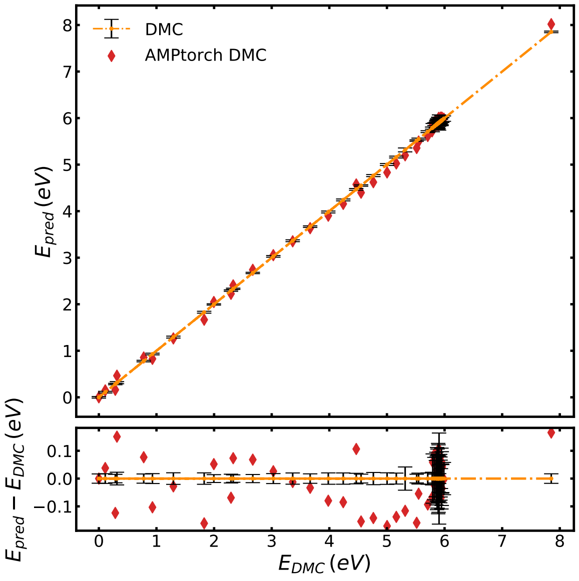


(c) (d)

**Figure S7:** Comparisons between the predicted and exact energies of $C_2$ from DFT, the AMPtorch DFT model without forces, DMC, and the AMPtorch DMC model. (a) Potential energy vs. C-C bond distance on the training data. (b) Potential energy vs. C-C bond distance predicted on the test data. (c) Parity plot comparing the DMC and predicted AMPtorch DMC energies as a function of the DMC energy on the training data. (d) Parity plot comparing the DMC and predicted AMPtorch DMC energies as a function of the DMC energy on the test data. The test data points are evenly distributed along the C-C bond distance, ranging from 0.93 Å to 4.28 Å.

## $H_2O$ Molecule MAE

The training dataset for $H_2O$ contains 12,000 ($20\times20\times30$) structures prepared by grid sampling 20 points along each of the two O-H bond distances and 30 points along the H-O-H bond angle. Points are taken within [0.7, 2.0) $\times R_0$, where $R_0 = 0.969$ Å is the equilibrium bond distance for each of the O-H bonds and within [0.3, 1.0)$\times 180^\circ$ for the bond angle. Test points were randomly selected within the same intervals for the test set.

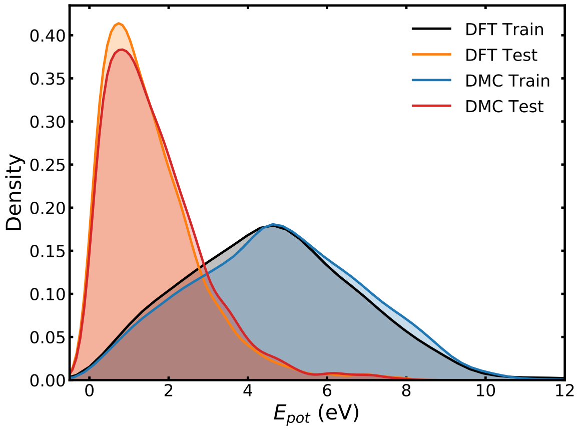


**Figure S8:** Energy distributions of the $H_2O$ training and test datasets for DFT and DMC, respectively. From the Figure, it can be observed that for both DFT and DMC, structures in the training dataset are more widely distributed in energy than those in the test dataset. This partially explains the larger MAEs values for the training dataset than the test dataset seen in Table S4.

Table S4 shows the training and test results of the DFT energy and force predictions for $H_2O$ from the AMPtorch DFT model, the AMPtorch DFT model without forces, and the AMPtorch DMC model.

**Table S4:** MAE on the training and test set energies and forces for $H_2O$. MAEs are provided for the three models discussed in this work: the AMPtorch DFT model with forces, the AMPtorch DFT model without forces, and the AMPtorch DMC model. For the DFT calculations, the reference data are DFT energies and forces. For the AMPtorch DMC model, the reference data are DMC energies.

| **MAE** | **AMPtorch DFT** (with forces) | **AMPtorch DFT** (without forces) | **AMPtorch DMC** |
|---|---|---|---|
| **Training Energies** MAE (eV/atom) | 0.0954 | 0.0917 | 0.0578 |
| **Training Forces** MAE (eV/(Å atom)) | 0.2592 | 0.5556 | - |
| **Test Energies** MAE (eV/atom) | 0.0104 | 0.0161 | 0.0164 |
| **Test Forces** MAE (eV/(Å atom)) | 0.0541 | 0.0992 | - |

## $CH_3Cl$ Molecule MAE

44,820 training points were extracted from the work by Owens *et al.*[2] Grid points were generated using energy-weighted Monte Carlo sampling in terms of nine internal coordinates: the C-Cl bond length $r_0$, with $1.3 \leq r_0 \leq 2.95$ Å; three C-H bond lengths $r_1$, $r_2$, and $r_3$, with $0.7 \leq r_i \leq 2.45$ Å; three $\angle$ $H_i$CCl interbond angles $\beta_1$, $\beta_2$, and $\beta_3$, with $65° \leq \beta_i \leq 165°$; and two dihedral angles $\tau_{12}$ and $\tau_{13}$ between adjacent planes containing $H_i$CCl and $H_j$CCl with $55° \leq \tau_{jk} \leq 185°$. A randomly sampled $CH_3Cl$ test set was generated within the same intervals. The energy distribution for both training dataset and test dataset are shown in Figure S9.

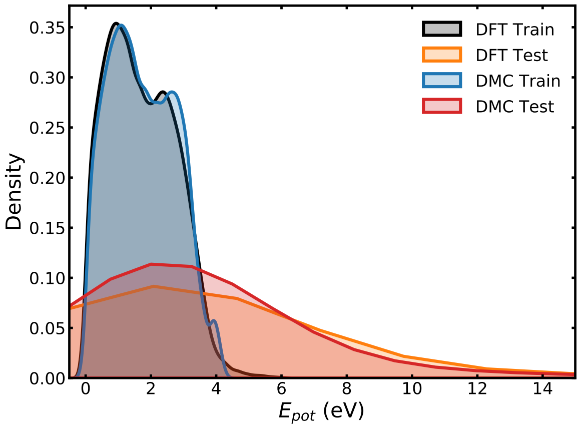


**Figure S9:** Energy distributions of the $CH_3Cl$ training and test datasets for DFT and DMC, respectively. The Figure shows that the training dataset is centered between 0 and 5 eV, while the test dataset has more points with larger potential energies. This difference results in the large MAE values for the AMPtorch models in test dataset.

Table S5 shows the training and test results of the DFT energy and force predictions for $CH_3Cl$ from the AMPtorch DFT models, and the AMPtorch DMC model.

**Table S5:** MAE on the training and test set energies and forces for $CH_3Cl$. MAEs are provided for the three models discussed in this work: the AMPtorch DFT model with forces, the AMPtorch DFT model without forces, and the AMPtorch DMC model. For the DFT calculations, the reference data are DFT energies and forces. For the AMPtorch DMC model, the reference data are DMC energies.

| **MAE** | **AMPtorch DFT** (with forces) | **AMPtorch DFT** (without forces) | **AMPtorch DMC** |
|---|---|---|---|
| **Training Energies** MAE (eV/atom) | 0.0005 | 0.0013 | 0.0030 |
| **Training Forces** MAE (eV/(Å atom)) | 0.0023 | 0.0103 | - |
| **Test Energies** MAE (eV/atom) | 0.3476 | 0.4478 | 0.8584 |
| **Test Forces** MAE (eV/(Å atom)) | 0.3470 | 0.4330 | - |

# Molecular Dynamics Data

## $C_2$ NVE and NVT Results

Figure S10 - S15 present the full trajectories of $C_2$ in the NVT and NVE ensembles. For comparison, we only show the first 120 fs of the trajectories for all models. However, the trajectories from the AMPtorch model can extend to 2 ps, which is indicative of the stability of the models.

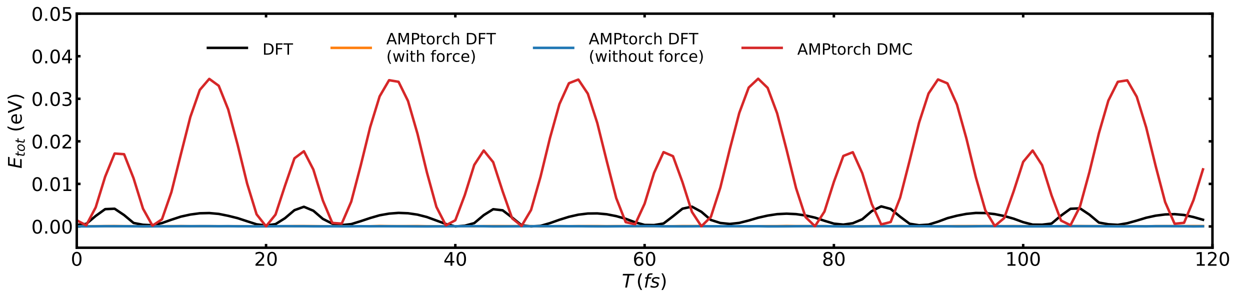


**(a)**

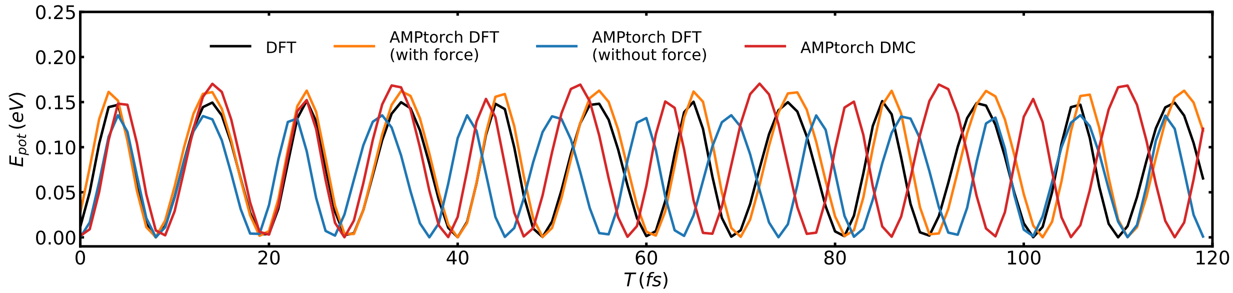


**(b)**

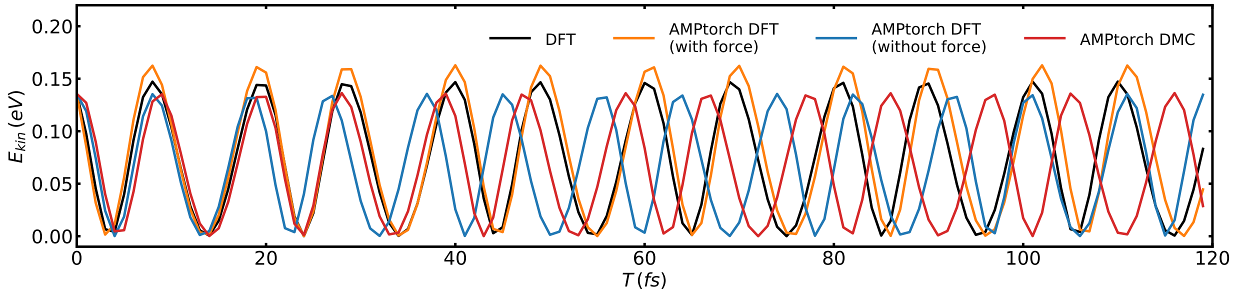


**(c)**

**Figure S10:** Energies vs. time for NVE molecular dynamics simulations of $C_2$ performed using DFT (black line), an AMPtorch model trained on DFT energies and forces (orange line), an AMPtorch model trained on DFT energies only (blue line), and an AMPtorch model trained with DMC energies only (red line). (a) Total energy, $E_{tot}$, vs. time. (b) Potential energy, $E_{pot}$, vs. time. (c) Kinetic energy, $E_{kin}$, vs. time.

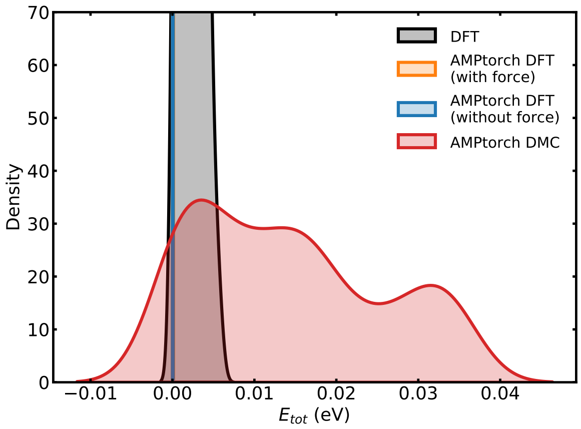


(a)

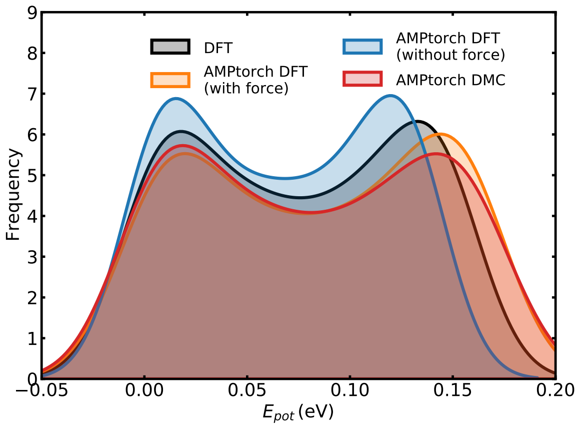


(b)

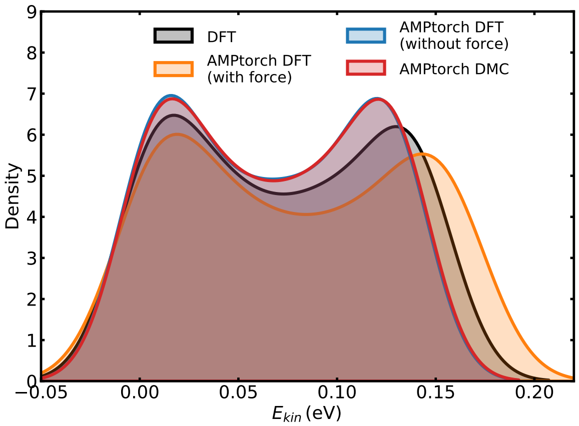


(c)

**Figure S11:** Energy distributions from $C_2$ NVE simulations performed using DFT, the AMPtorch DFT (with forces) model, the AMPtorch DFT (without forces) model, and the AMPtorch DMC model. (a) Density vs. total energy. (b) Density vs. potential energy. (c) Density vs. kinetic energy.

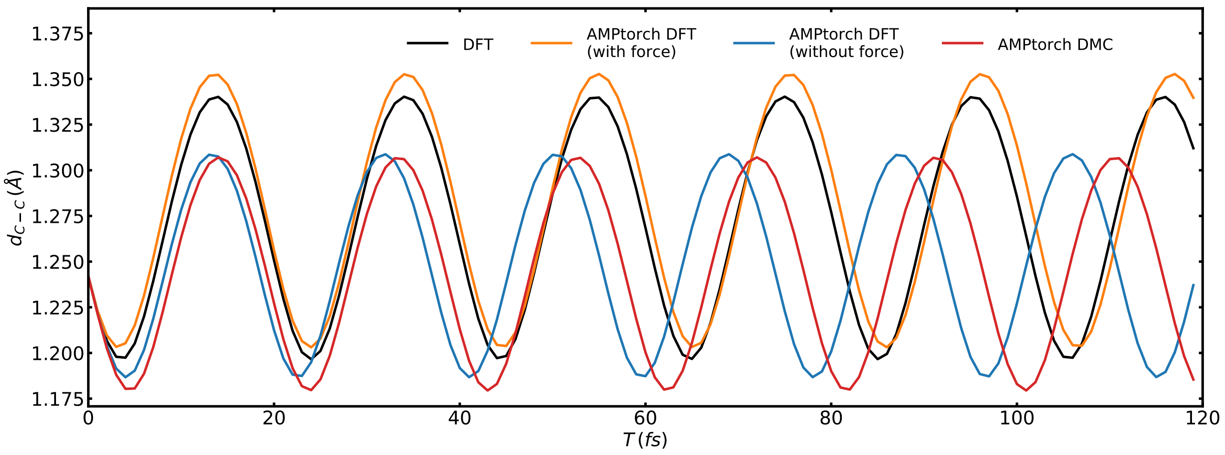


**(a)**

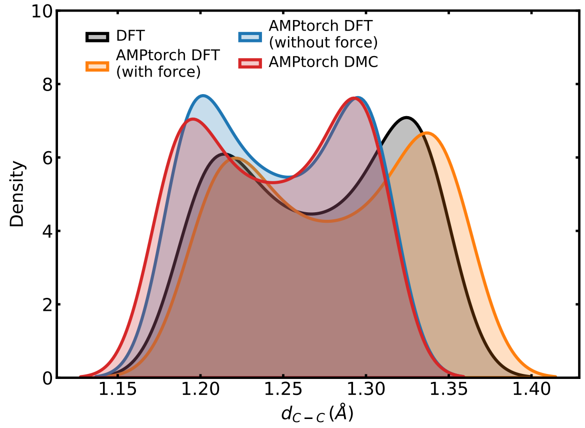


**(b)**

**Figure S12:** Bond distances for NVE molecular dynamics simulations of $C_2$ performed using DFT (black line), an AMPtorch model trained on DFT energies and forces (orange line), an AMPtorch model trained on DFT energies only (blue line), and an AMPtorch model trained with DMC energies only (red line). (a) $d_{C-C}$ bond distance vs. time. (b) $d_{C-C}$ bond distance distribution.

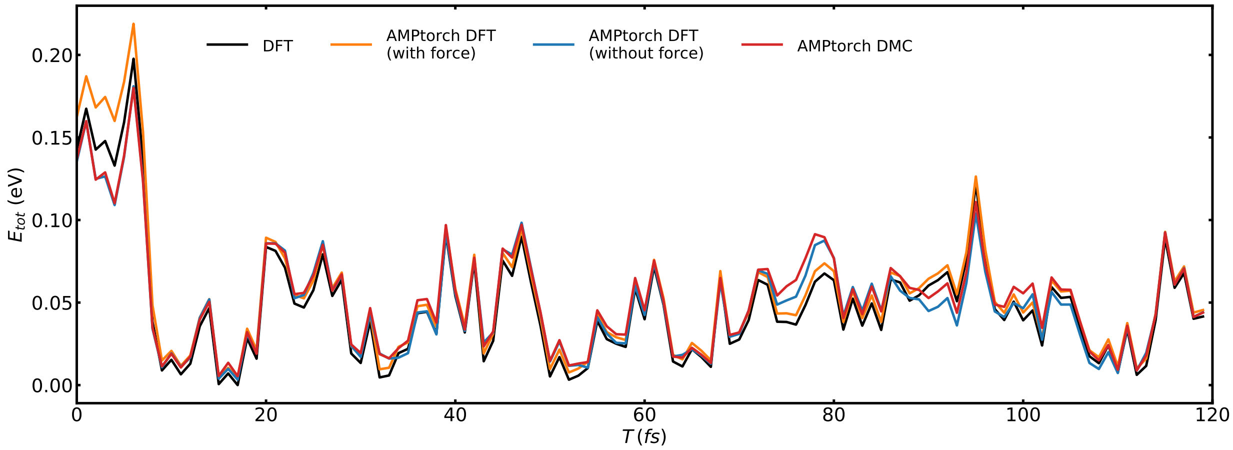


**(a)**

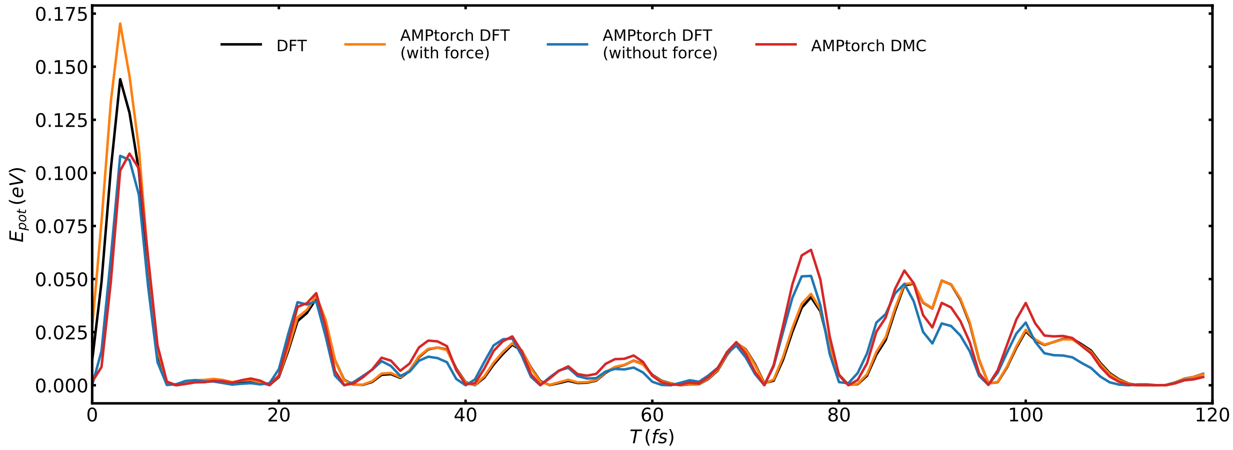


**(b)**

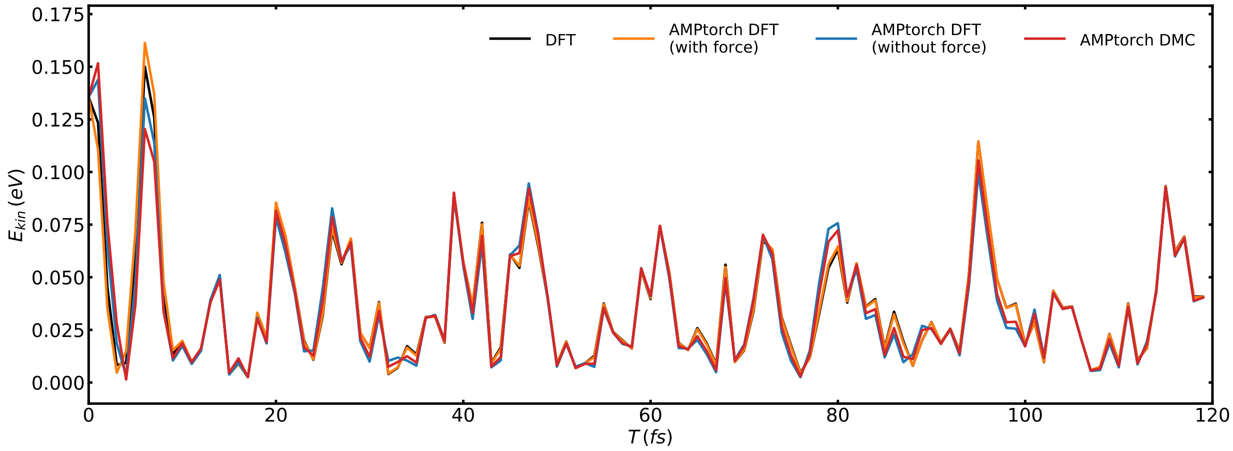


**(c)**

**Figure S13:** Energies vs. time for NVT molecular dynamics simulations of $C_2$ performed using DFT (black line), an AMPtorch model trained on DFT energies and forces (orange line), an AMPtorch model trained on DFT energies only (blue line), and an AMPtorch model trained with DMC energies only (red line). (a) Total energy, $E_{tot}$, vs. time. (b) Potential energy, $E_{pot}$, vs. time. (c) Kinetic energy, $E_{kin}$, vs. time.

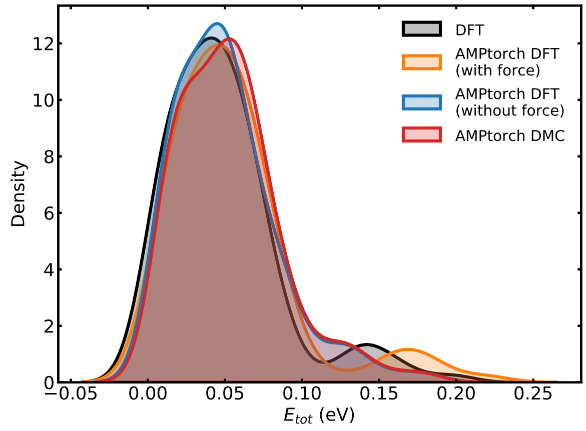


**(a)**

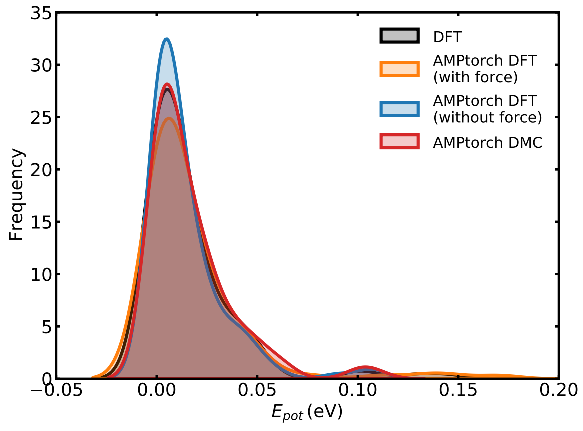


**(b)**

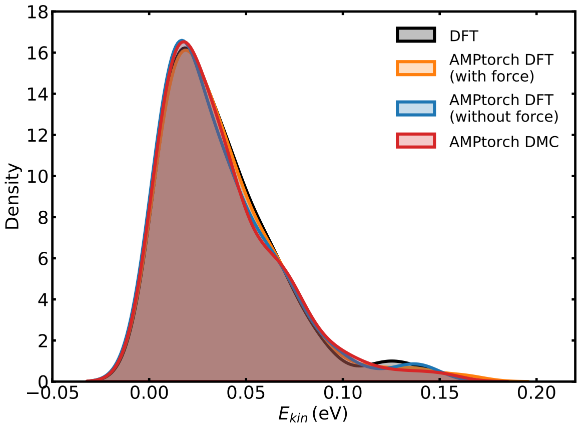


**(c)**

**Figure S14:** Energy distributions from $C_2$ NVT simulations performed using DFT, the AMPtorch DFT (with forces) model, the AMPtorch DFT (without forces) model, and the AMPtorch DMC model. (a) Density vs. total energy. (b) Density vs. potential energy. (c) Density vs. kinetic energy.

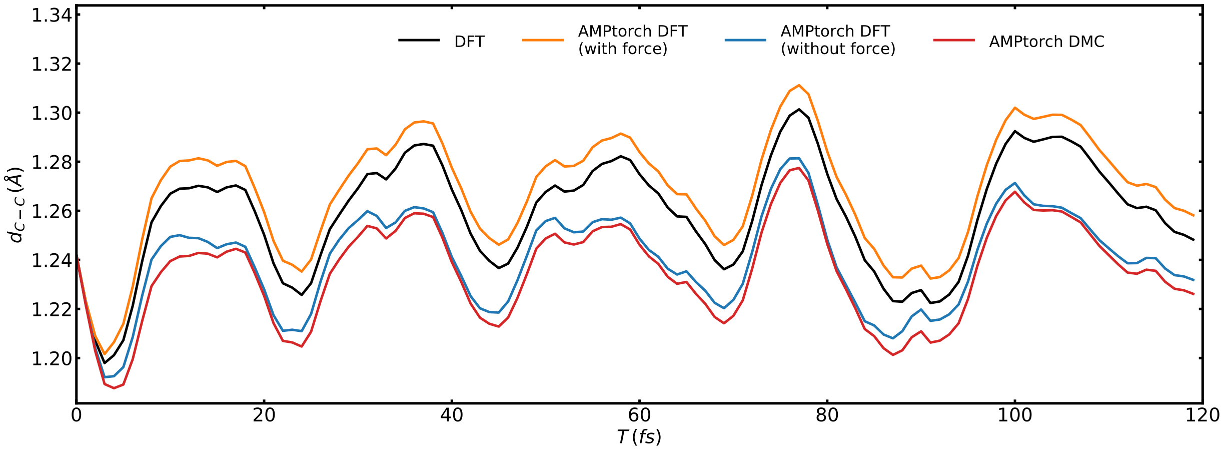


**(a)**

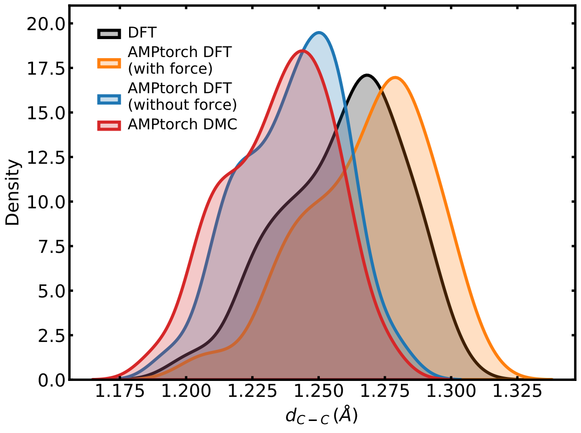


**(b)**

**Figure S15:** Bond distances for NVT molecular dynamics simulations of $C_2$ performed using DFT (black line), an AMPtorch model trained on DFT energies and forces (orange line), an AMPtorch model trained on DFT energies only (blue line), and an AMPtorch model trained with DMC energies only (red line). (a) $d_{C-C}$ bond distance vs. time. (b) $d_{C-C}$ bond distance distribution.

# $H_2O$ NVE and NVT Results

In this section, we present the total ($E_{tot}$), potential ($E_{pot}$), and kinetic ($E_{kin}$) energies vs. time from DFT and our model calculations for $H_2O$ modeled in the NVE and NVT ensembles. These curves attest to how well these models conserve and redistribute energy among the molecular modes.

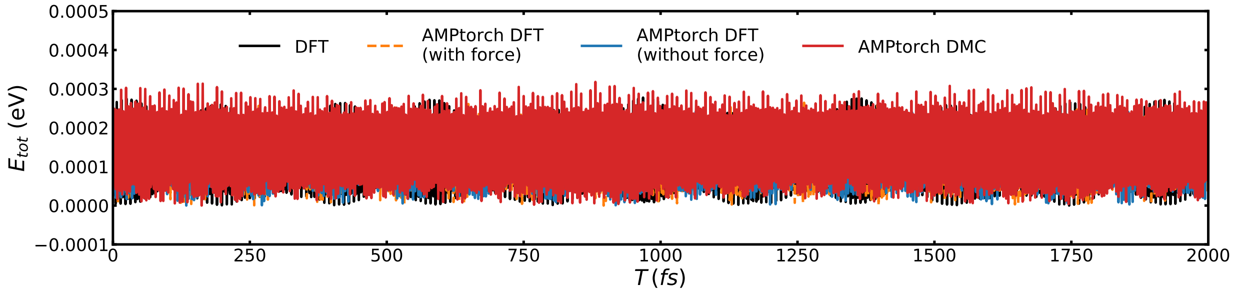


**(a)**

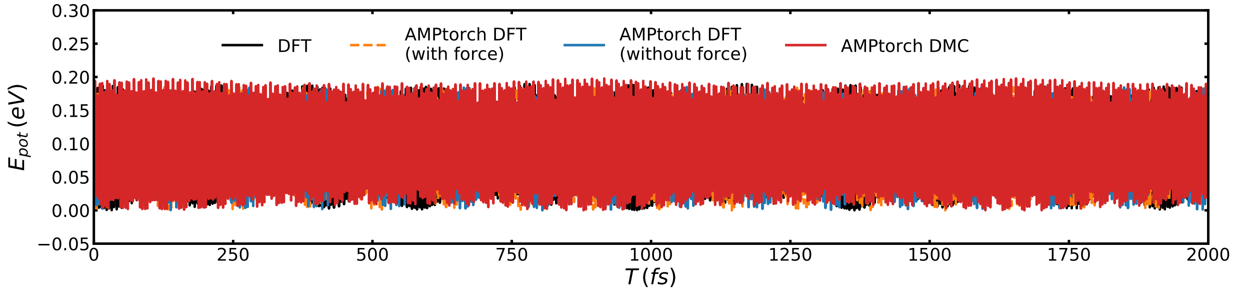


**(b)**

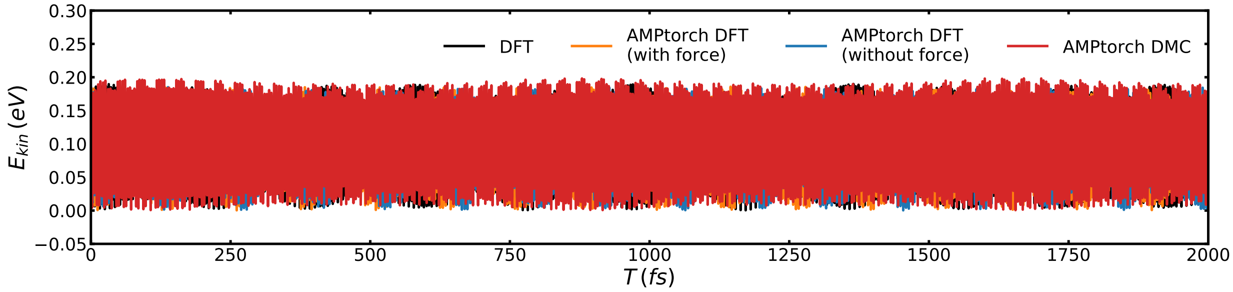


**(c)**

**Figure S16:** Energies vs. time for NVE molecular dynamics simulations of $H_2O$ performed using DFT (black line), an AMPtorch model trained on DFT energies and forces (orange line), an AMPtorch model trained on DFT energies only (blue line), and an AMPtorch model trained on DMC energies only (red line). (a) Total energy, $E_{tot}$, vs. time. (b) Potential energy, $E_{pot}$, vs. time. (c) Kinetic energy, $E_{kin}$, vs. time.

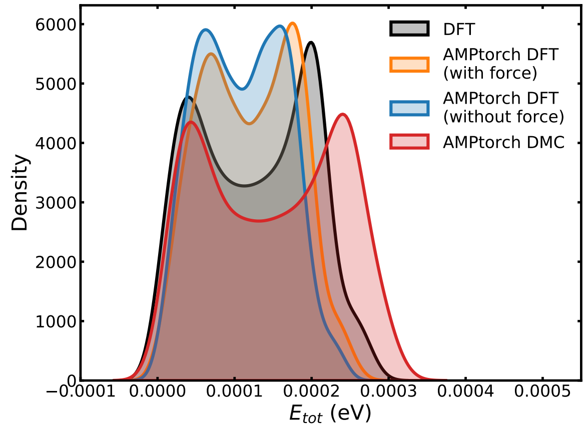


**(a)**

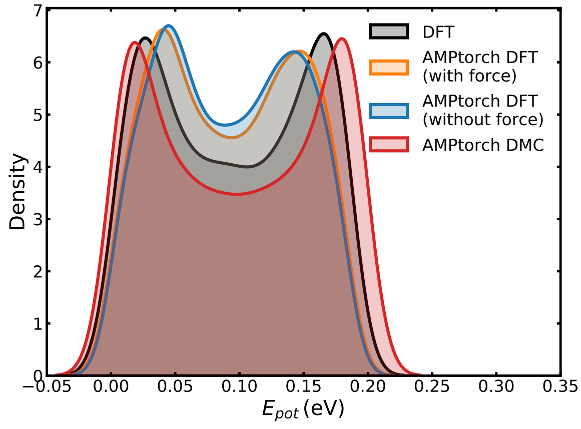


**(b)**

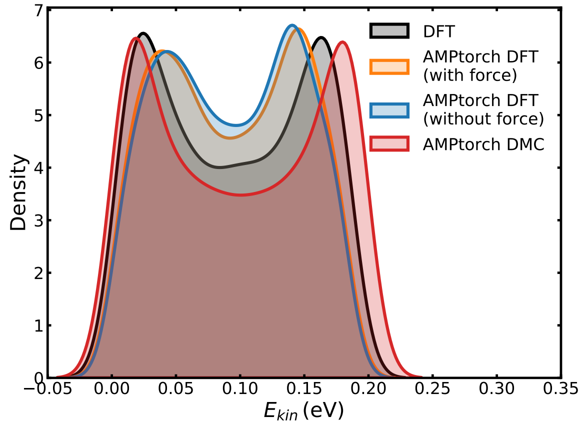


**(c)**

**Figure S17:** Energy distributions from $H_2O$ NVE simulations performed using DFT (black line), the AMPtorch DFT (with forces) model (orange line), the AMPtorch DFT (without forces) model (blue line), and the AMPtorch DMC model (red line). (a) Density vs. total energy. (b) Density vs. potential energy. (c) Density vs. kinetic energy.

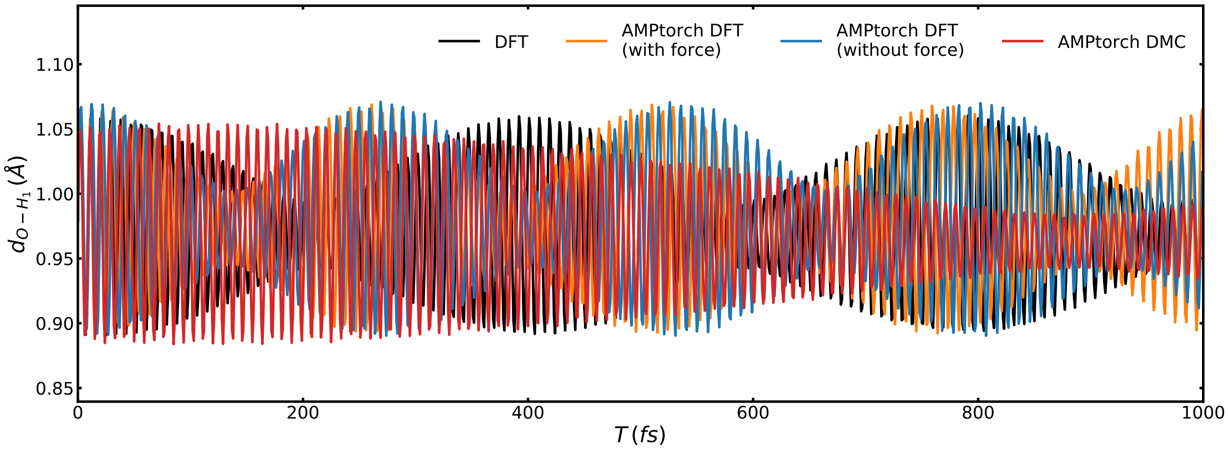


**(a)**

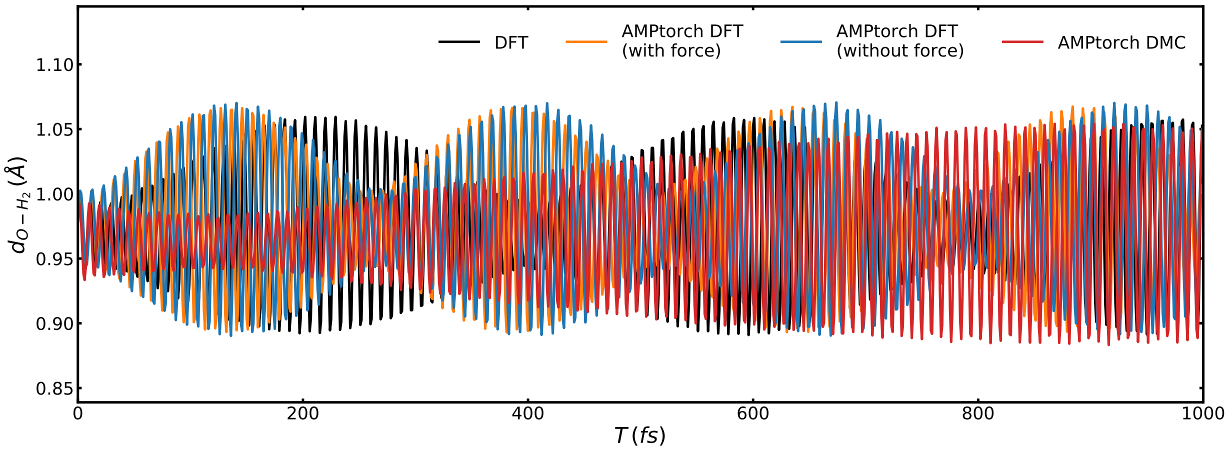


**(b)**

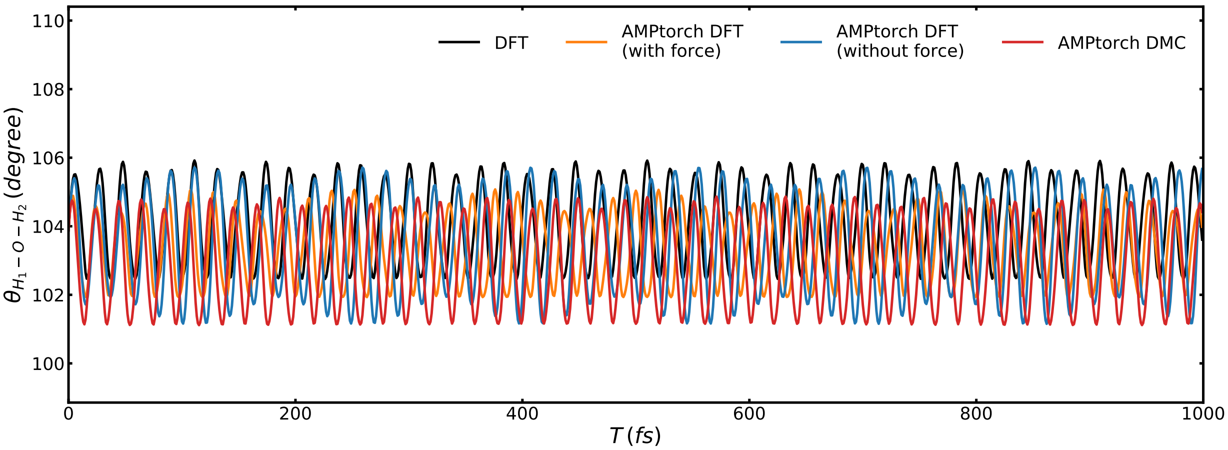


**(c)**

**Figure S18:** Bond distances and angles for NVE molecular dynamics simulations of $H_2O$ performed using DFT (black line), an AMPtorch model trained on DFT energies and forces (orange line), an AMPtorch model trained on DFT energies only (blue line), and an AMPtorch model trained with DMC energies only (red line). (a) $d_{O-H_1}$ bond distance vs. time. (b) $d_{O-H_2}$ bond distance vs. time. (c) $\theta_{H_1-O-H_2}$ bond angle vs. time.

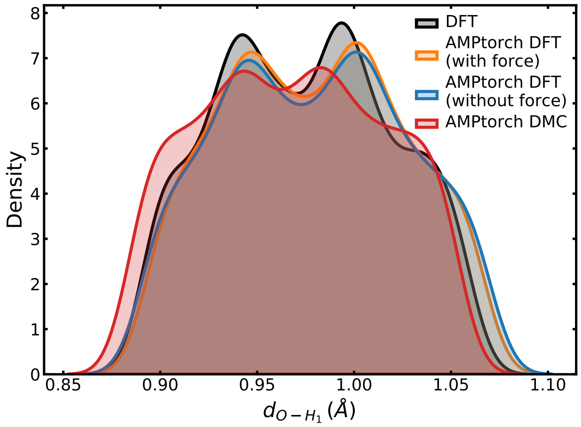


**(a)**

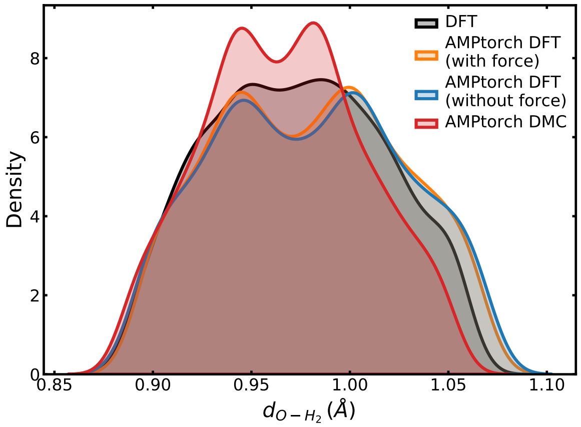


**(b)**

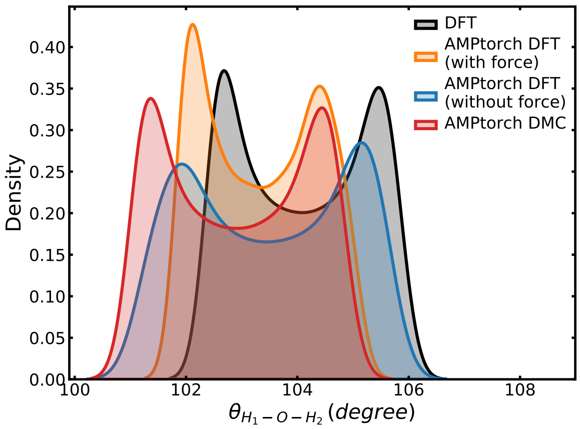


**(c)**

**Figure S19:** Bond distance and angle distributions from $H_2O$ NVE simulations performed using DFT, the AMPtorch DFT (with forces) model, the AMPtorch DFT (without forces) model, and the AMPtorch DMC model. While the bond angle distributions for the AMPtorch DFT (without forces) and AMPtorch DMC models are much broader than those for DFT and the AMPtorch DFT (with force) model, the bond distance distributions are closer to each other. This is likely due to the fact that the bond angle potential energy well is shallower than the bond distance well.

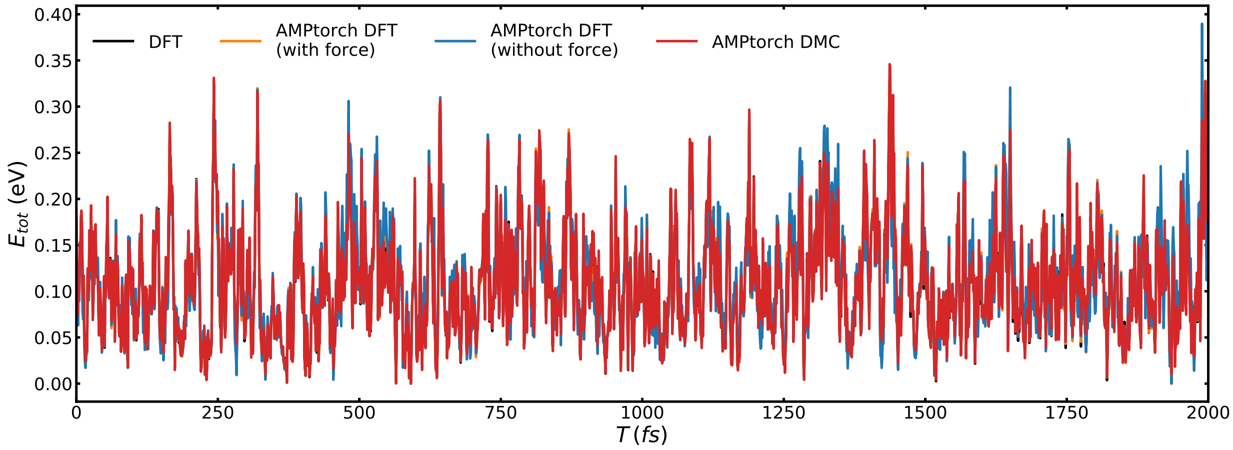


**(a)**

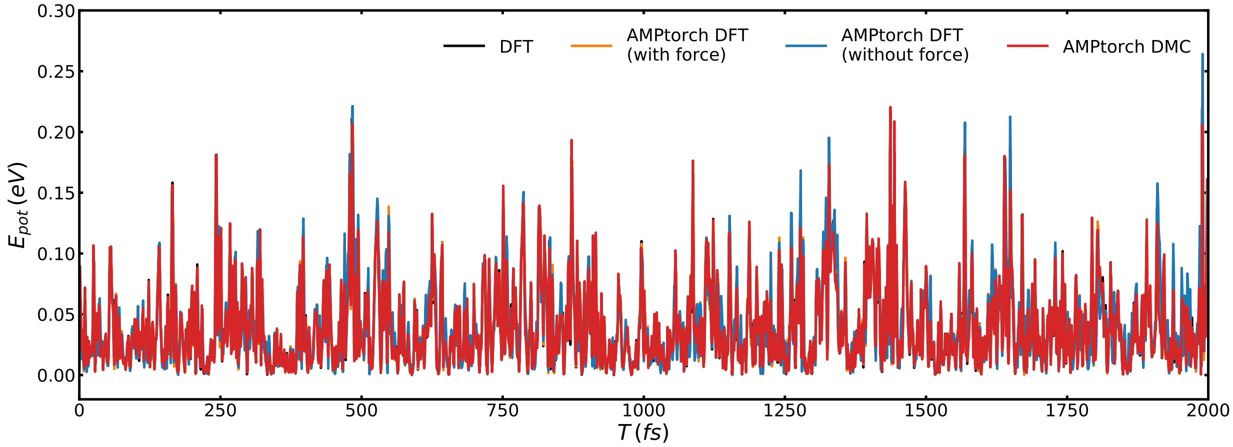


**(b)**

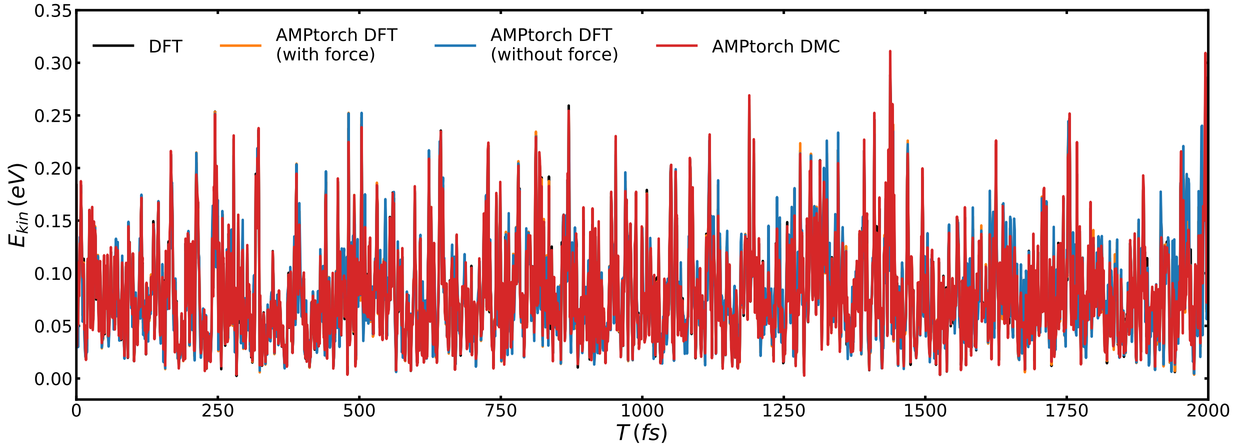


**(c)**

**Figure S20:** Energies vs. time for NVT molecular dynamics simulations of $H_2O$ performed using DFT (black line), an AMPtorch model trained on DFT energies and forces (orange line), an AMPtorch model trained on DFT energies only (blue line), and an AMPtorch model trained with DMC energies only (red line). (a) Total energy, $E_{tot}$ vs. time; (b) Potential energy, $E_{pot}$ vs. time; and (c) Kinetic energy, $E_{kin}$ vs. time.

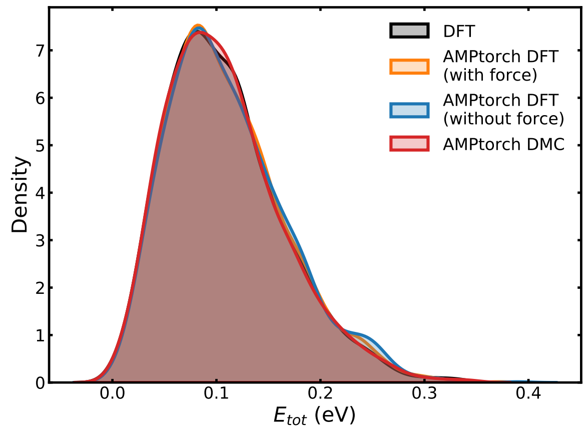


**(a)**

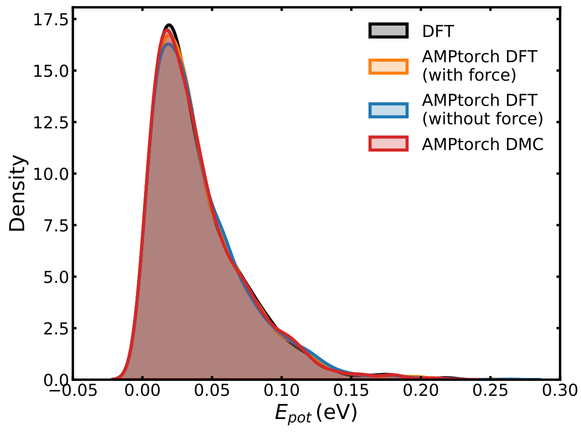


**(b)**

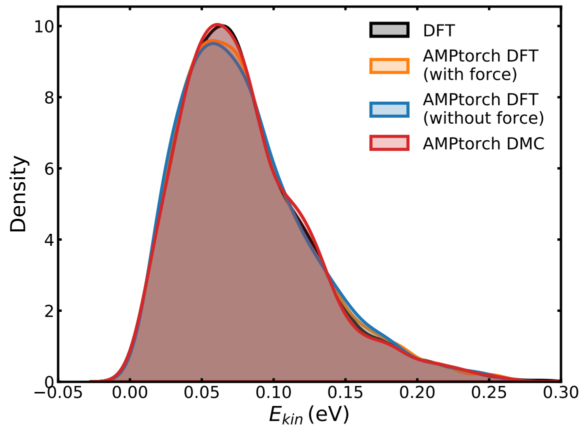


**(c)**

**Figure S21:** Energy distributions from $H_2O$ NVT simulations performed using DFT, the AMPtorch DFT (with forces) model, the AMPtorch DFT (without forces) model, and the AMPtorch DMC model. (a) Density vs. total energy; (b) Density vs. potential energy; and (c) Density vs. kinetic energy.

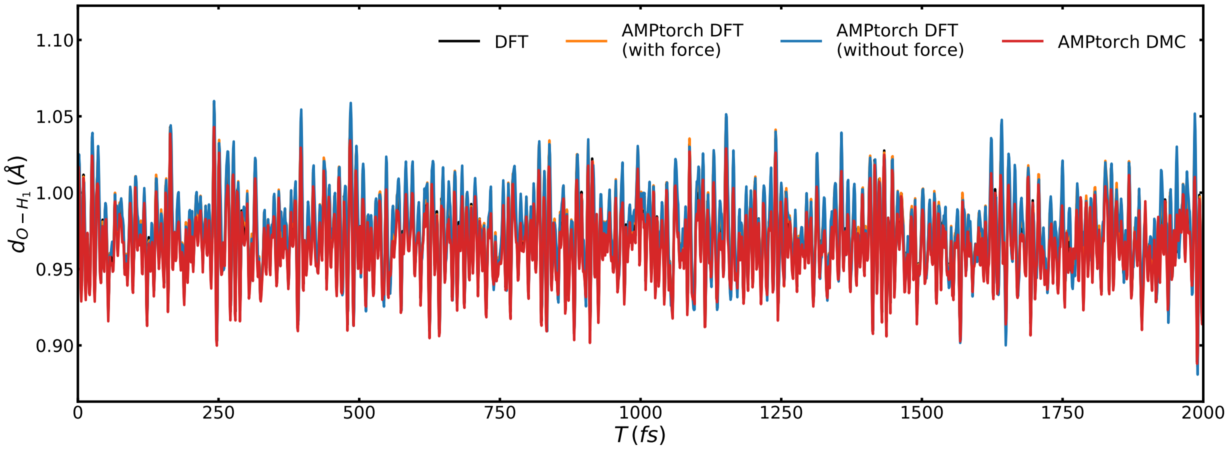


**(a)**

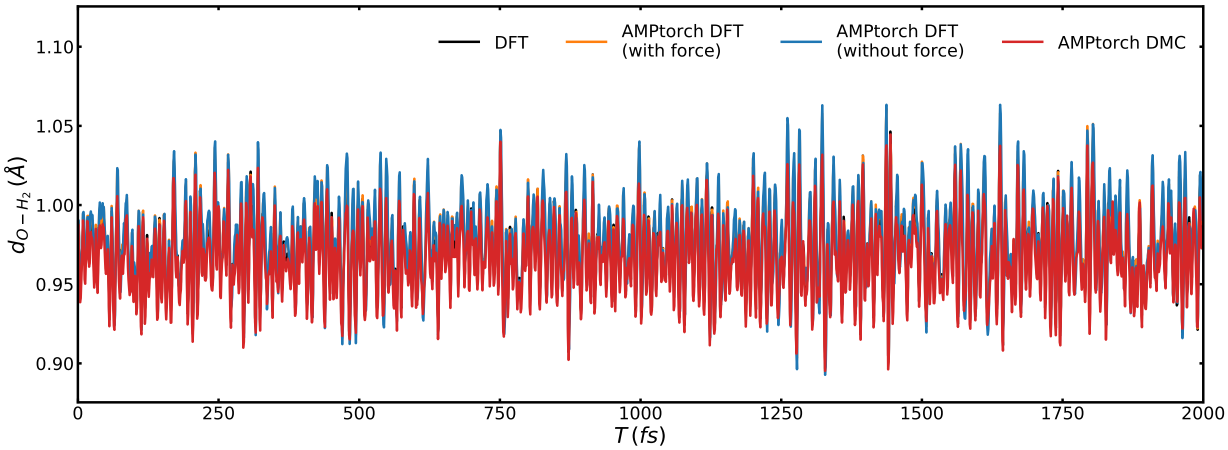


**(b)**

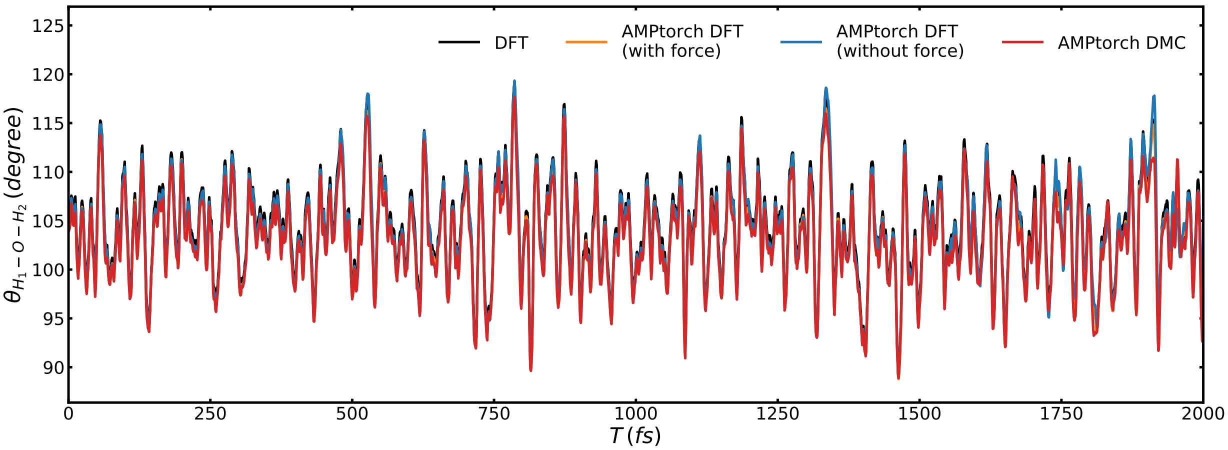


**(c)**

**Figure S22:** Bond distances and angles vs. time for NVT molecular dynamics simulations of $H_2O$ performed using DFT (black line), an AMPtorch model trained on DFT energies and forces (orange line), an AMPtorch model trained on DFT energies only (blue line), and an AMPtorch model trained with DMC energies only (red line). (a) First O-H bond distance vs. time; (b) second O-H bond distance vs. time; and (c) bond angle vs. time.

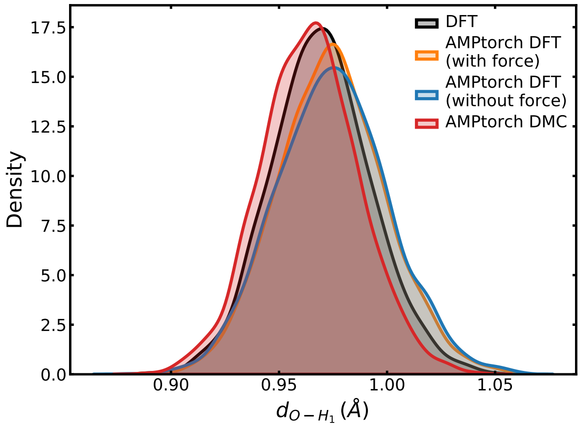


**(a)**

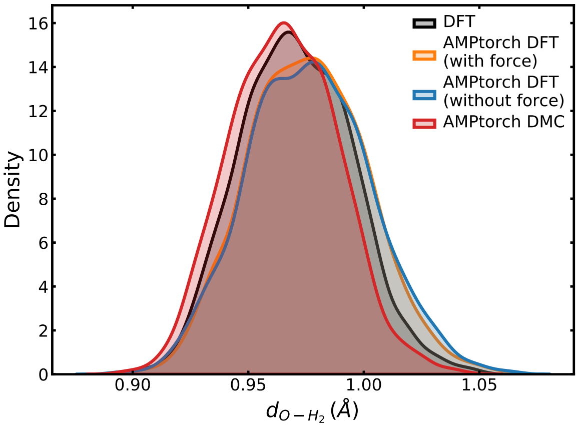


**(b)**

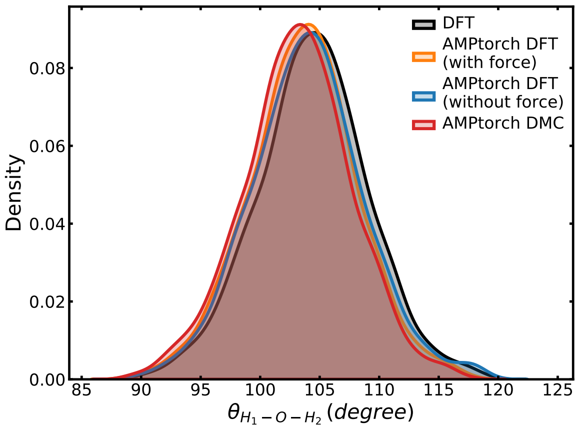


**(c)**

**Figure S23: Observables distributions** from $H_2O$ NVT simulation performed by DFT, AMPtorch DFT (with forces), AMPtorch DFT (without forces) and AMPtorch DMC. While the bond angle distributions for AMPtorch DFT (without forces) and AMPtorch DMC are much broader than the DFT and AMPtorch DFT (with forces) models, the bond distance distributions are closer to each other. The reason might be that the potential well is shallower for the bond angle than the bond distance.

# $CH_3Cl$ NVE and NVT Results

In this section, we present the total ($E_{tot}$), potential ($E_{pot}$), and kinetic ($E_{kin}$) energies vs. time from DFT and our model calculations for $H_2O$ modeled in the NVE and NVT ensembles. These curves attest to how well these models conserve and redistribute energy among the molecular modes.

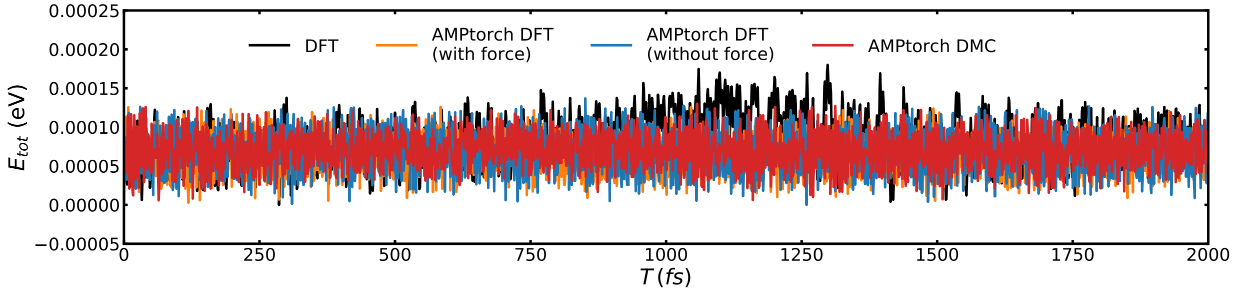


**(a)**

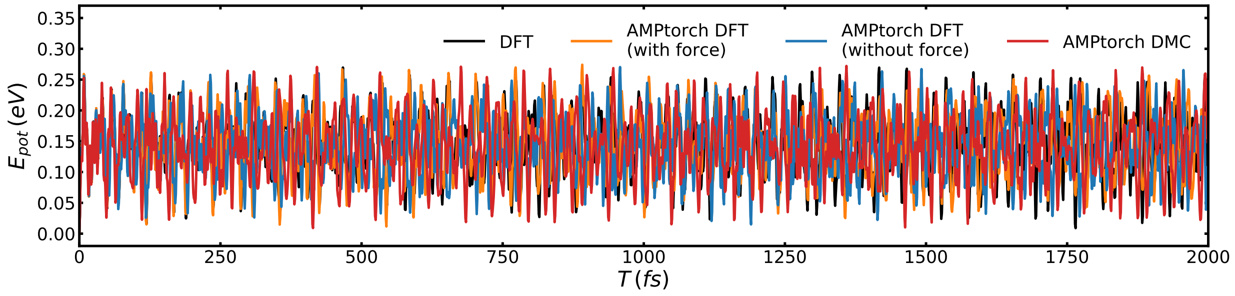


**(b)**

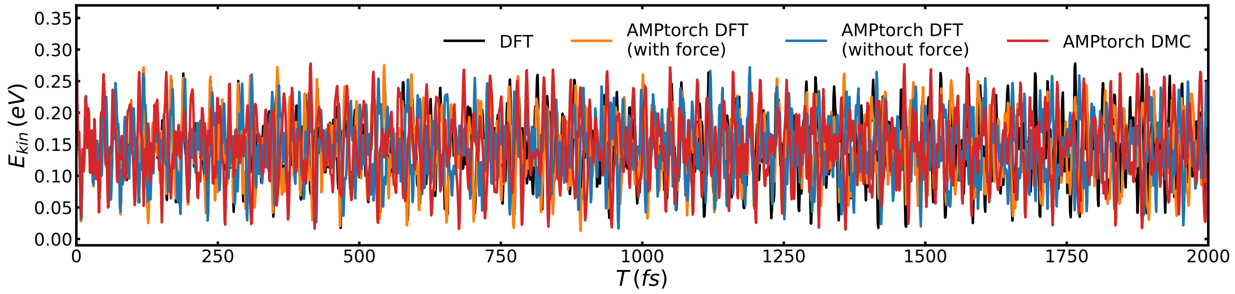


**(c)**

**Figure S24:** Energies vs. time for $CH_3Cl$ during MD simulations in the NVE ensemble using DFT, AMPtorch DFT (with forces), AMPtorch DFT (without forces), and AMPtorch DMC. (a) Total energy vs. time; (b) Potential energy vs. time; (c) Kinetic energy vs. time.

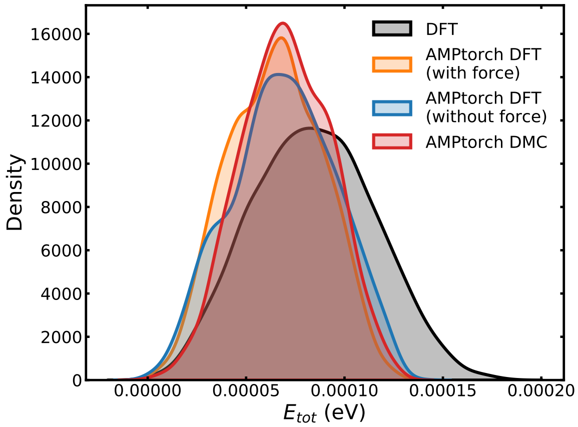


**(a)**

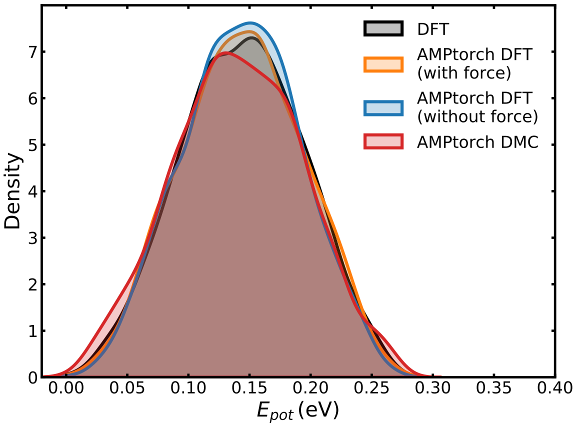


**(b)**

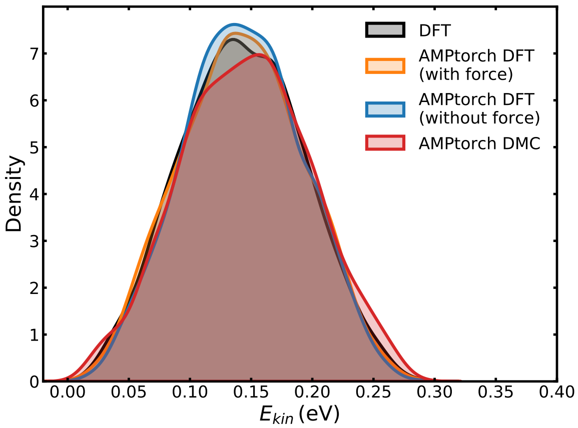


**(c)**

**Figure S25:** Energy distributions from $CH_3Cl$ NVE simulations performed using DFT, the AMPtorch DFT (with forces) model, the AMPtorch DFT (without forces) model, and the AMPtorch DMC model. (a) Density vs. total energy; (b) Density vs. potential energy; and (c) Density vs. kinetic energy.

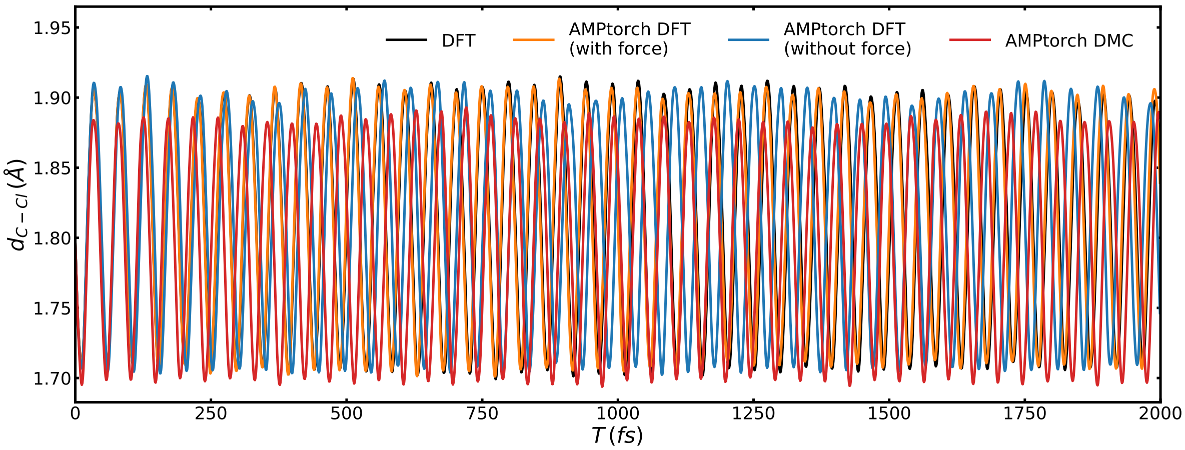


**(a)**

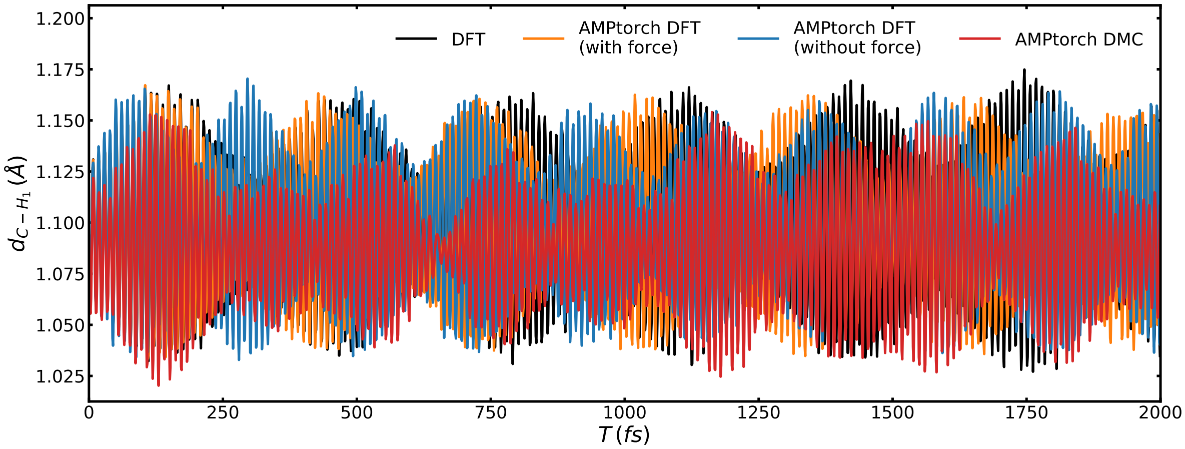


**(b)**

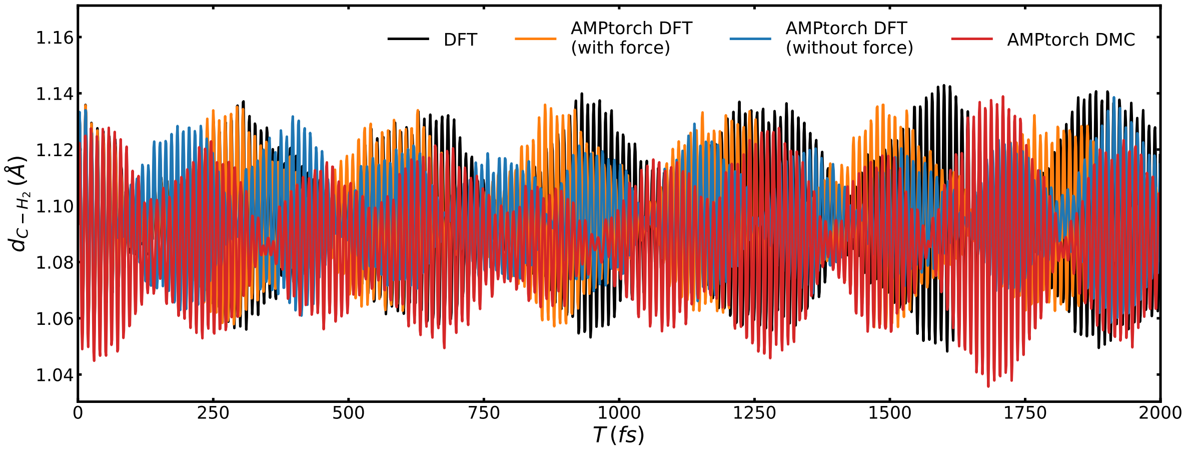


**(c)**

**Figure S26:** Select bond distances vs. time for $CH_3Cl$ during MD simulations in the NVE ensemble using DFT, AMPtorch DFT (with forces), AMPtorch DFT (without forces), and AMPtorch DMC.

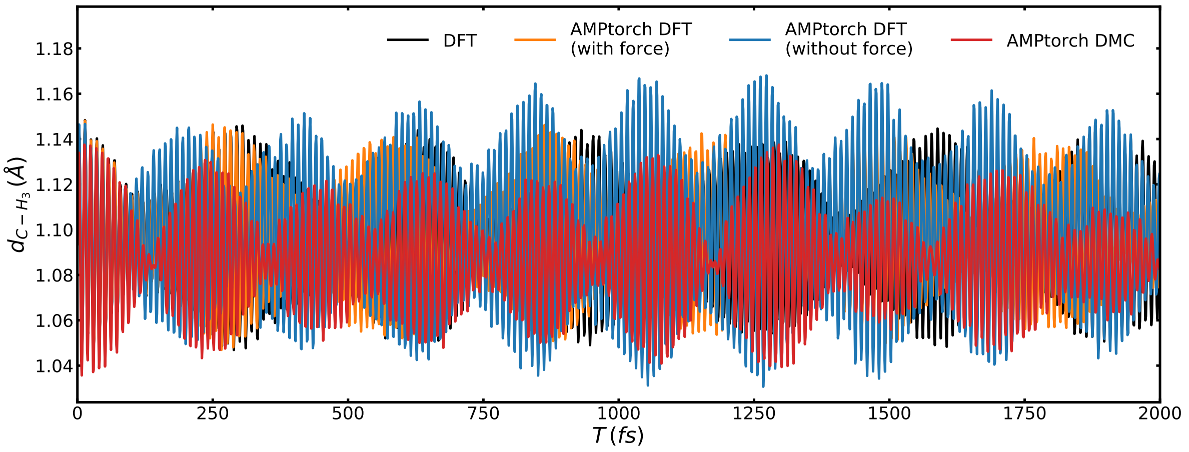


**(a)**

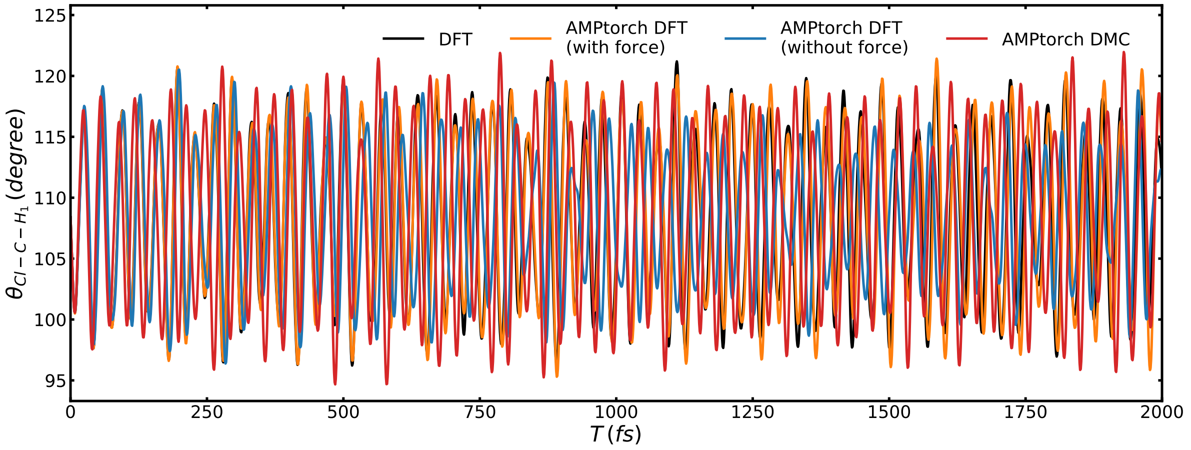


**(b)**

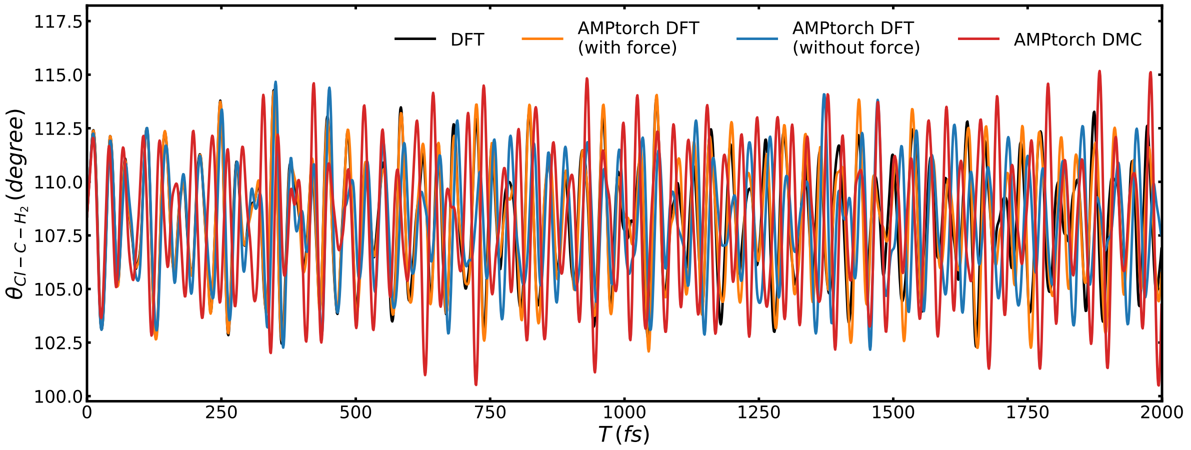


**(c)**

**Figure S27:** Select bond distances and angles vs. time for $CH_3Cl$ during MD simulations in the NVE ensemble using DFT, AMPtorch DFT (with forces), AMPtorch DFT (without forces), and AMPtorch DMC.

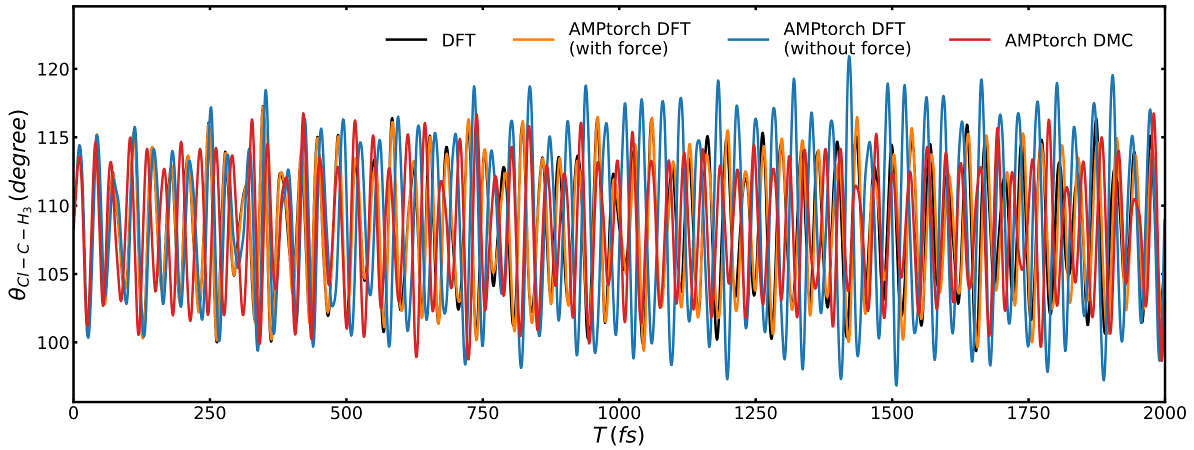


**(a)**

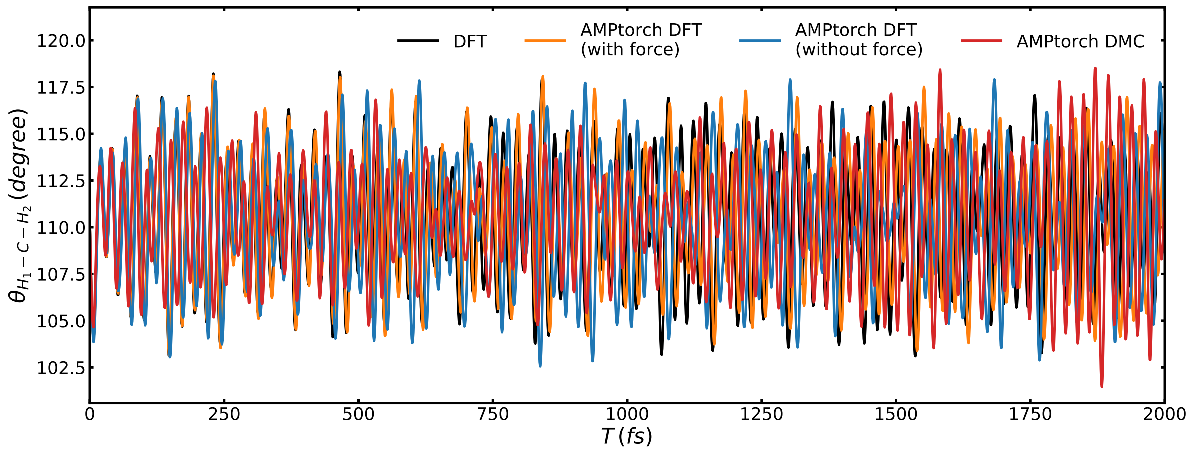


**(b)**

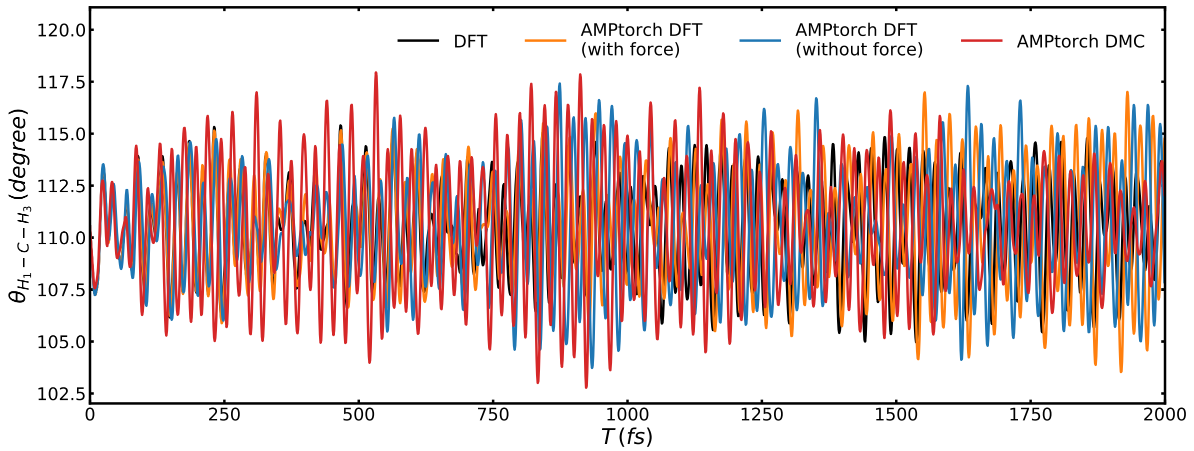


**(c)**

**Figure S28:** Select bond angles vs. time for $CH_3Cl$ during MD simulations in the NVE ensemble using DFT, AMPtorch DFT (with forces), AMPtorch DFT (without forces), and AMPtorch DMC.

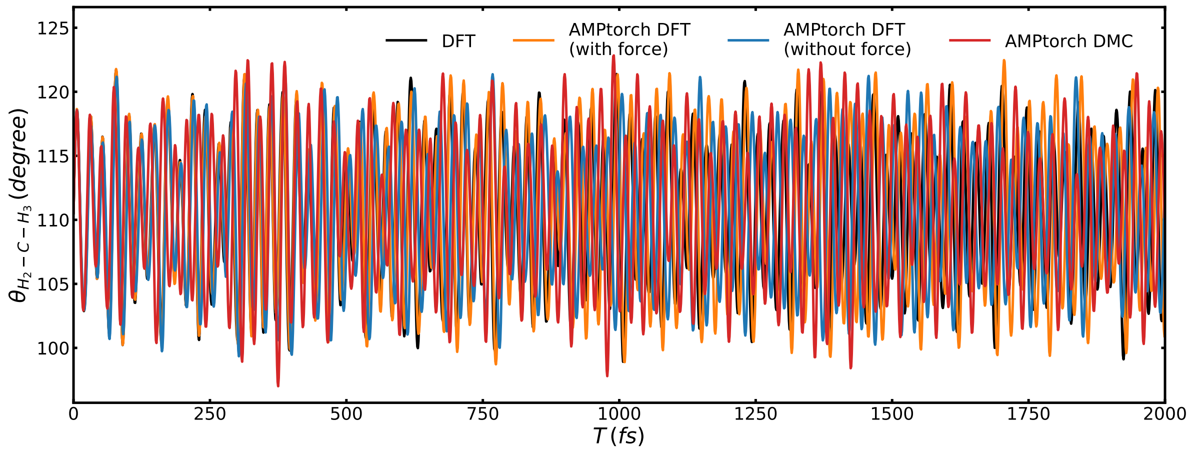


**(a)**

**Figure S29:** Last bond angle vs. time for $CH_3Cl$ during MD simulations in the NVE ensemble using DFT, AMPtorch DFT (with forces), AMPtorch DFT (without forces), and AMPtorch DMC.

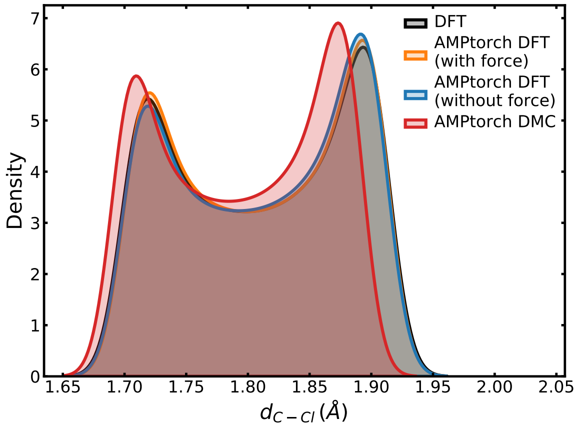


**(a)**

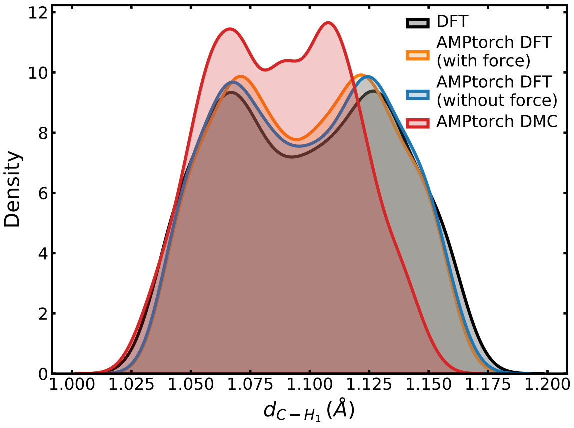


**(b)**

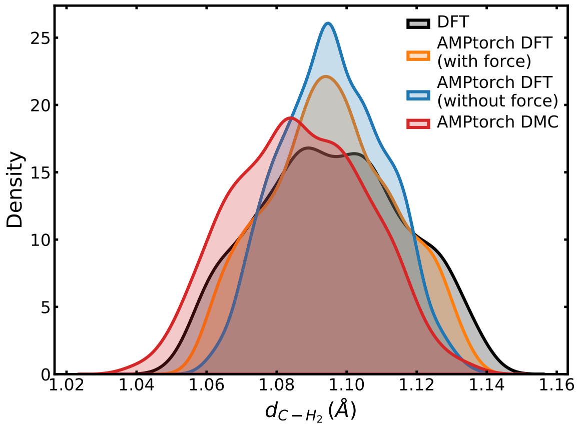


**(c)**

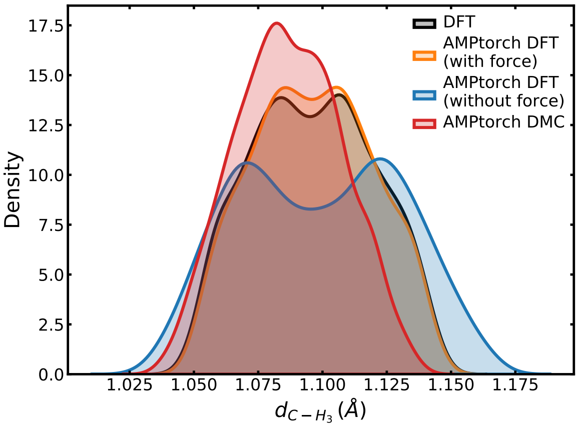


**(d)**

**Figure S30:** Bond distance distributions from $CH_3Cl$ NVE simulation performed by DFT, AMPtorch DFT (with forces), AMPtorch DFT (without forces) and AMPtorch DMC. (a) Density vs. C-Cl bond distance; (b) Density vs. C-$H_1$ bond distance; (c) Density vs. C-$H_2$ bond distance; and (d) Density vs. C-$H_3$ bond distance.

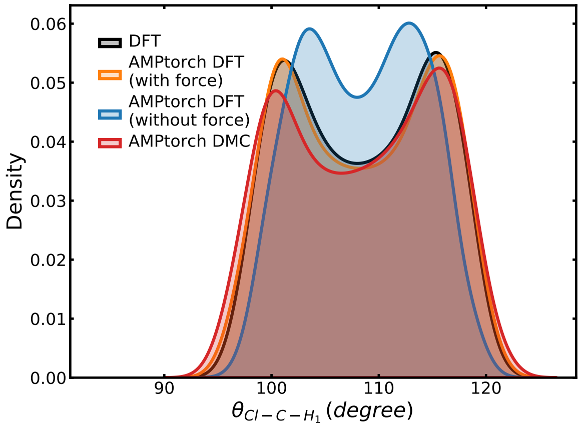


**(a)**

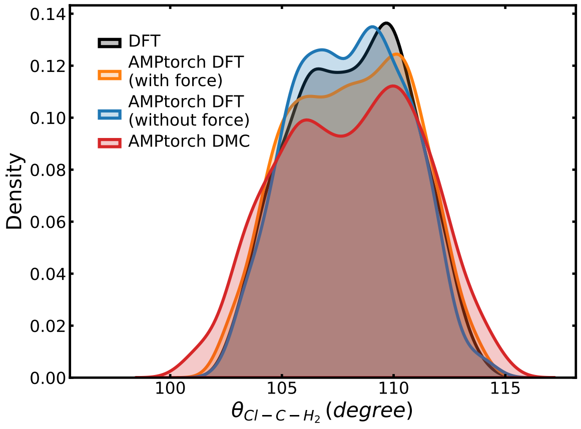


**(b)**

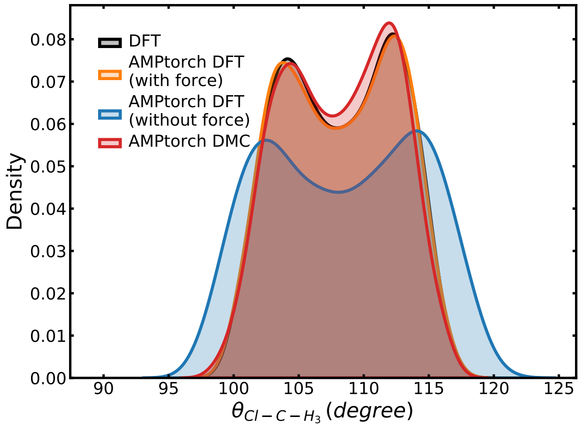


**(c)**

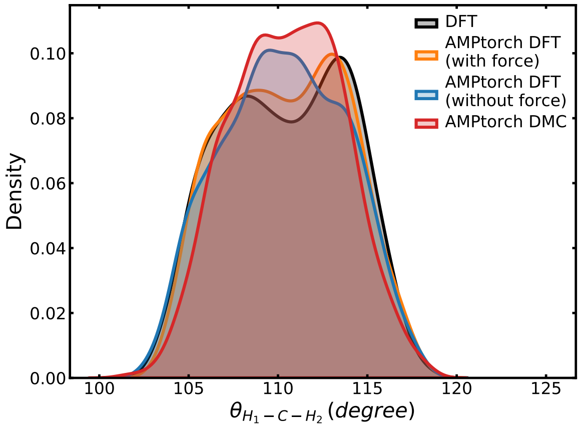


**(d)**

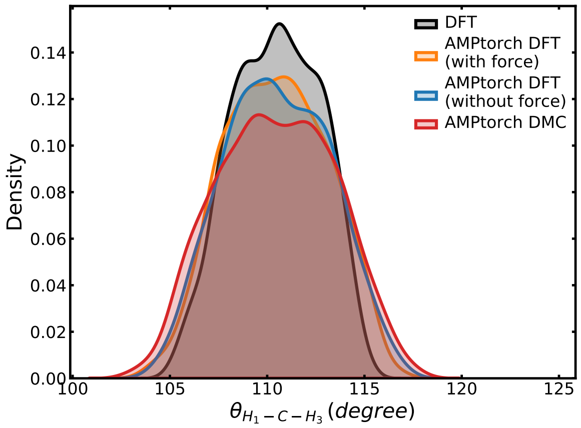


**(e)**

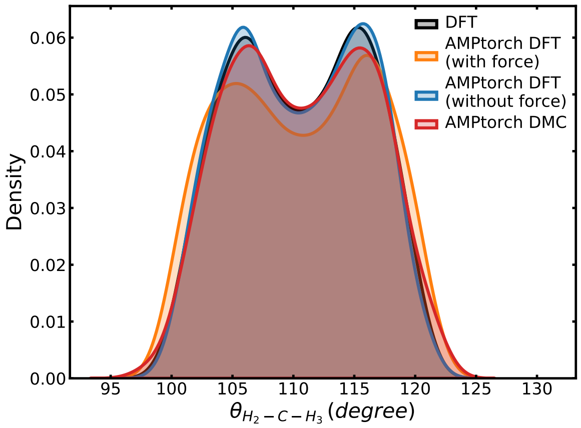


**(f)**

**Figure S31:** Bond angle distributions from $CH_3Cl$ NVE simulations performed using DFT, AMPtorch DFT (with forces), AMPtorch DFT (without forces), and AMPtorch DMC. (a) Density vs. Cl-C-$H_1$ bond angle; (b) Density vs. Cl-C-$H_2$ bond angle; (c) Density vs. Cl-C-$H_3$ bond angle; (d) Density vs. $H_1$-C-$H_2$ bond angle; (e) Density vs. $H_1$-C-$H_3$ bond angle; (f) Density vs. $H_2$-C-$H_3$ bond angle.

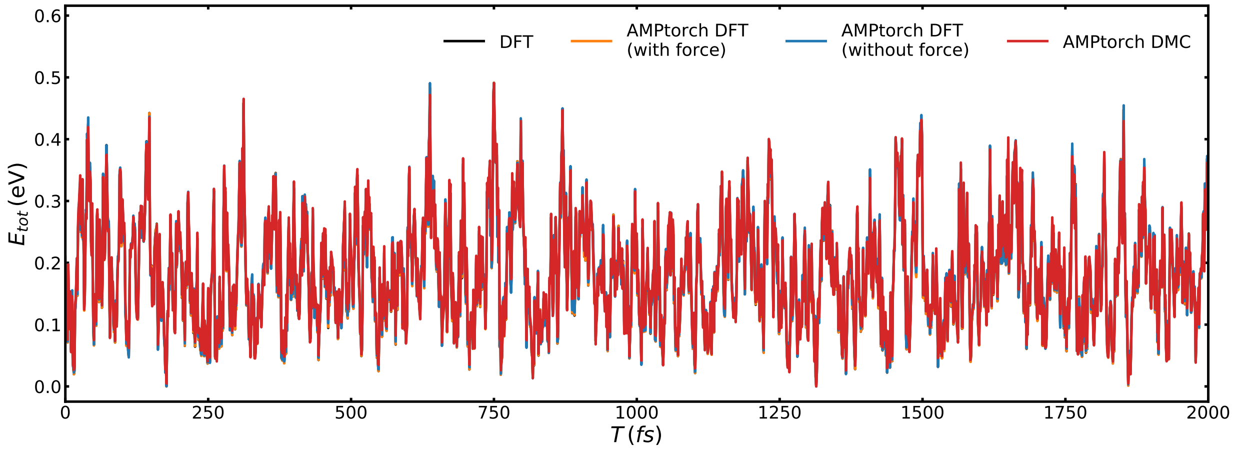


**(a)**

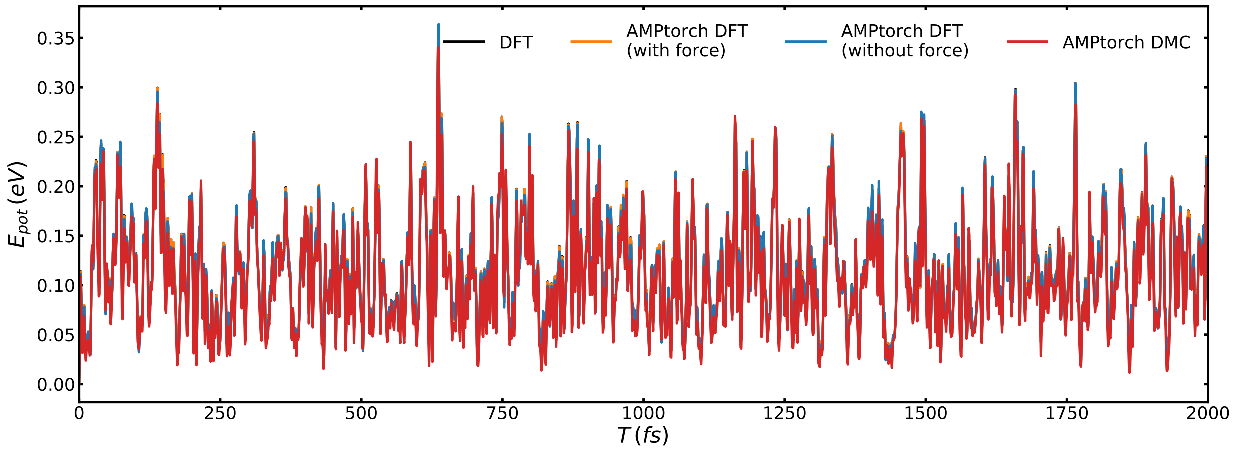


**(b)**

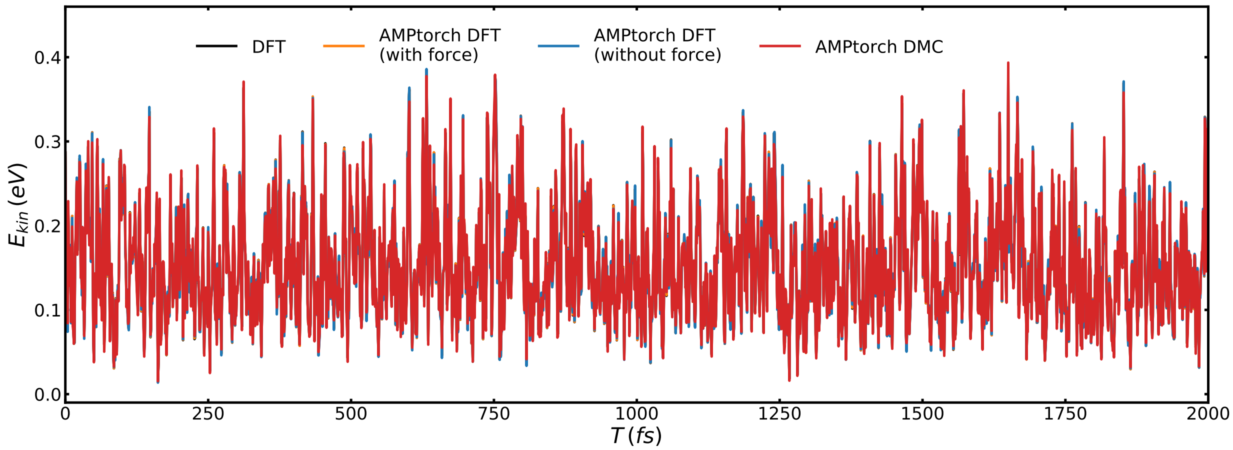


**(c)**

**Figure S32:** Energies vs. time for $CH_3Cl$ during MD simulations in the canonical (NVT) ensemble using DFT, AMPtorch DFT (with forces), AMPtorch DFT (without forces) and AMPtorch DMC. (a) Total energy vs. time. (b) Potential energy vs. time. (c) Kinetic energy vs. time.

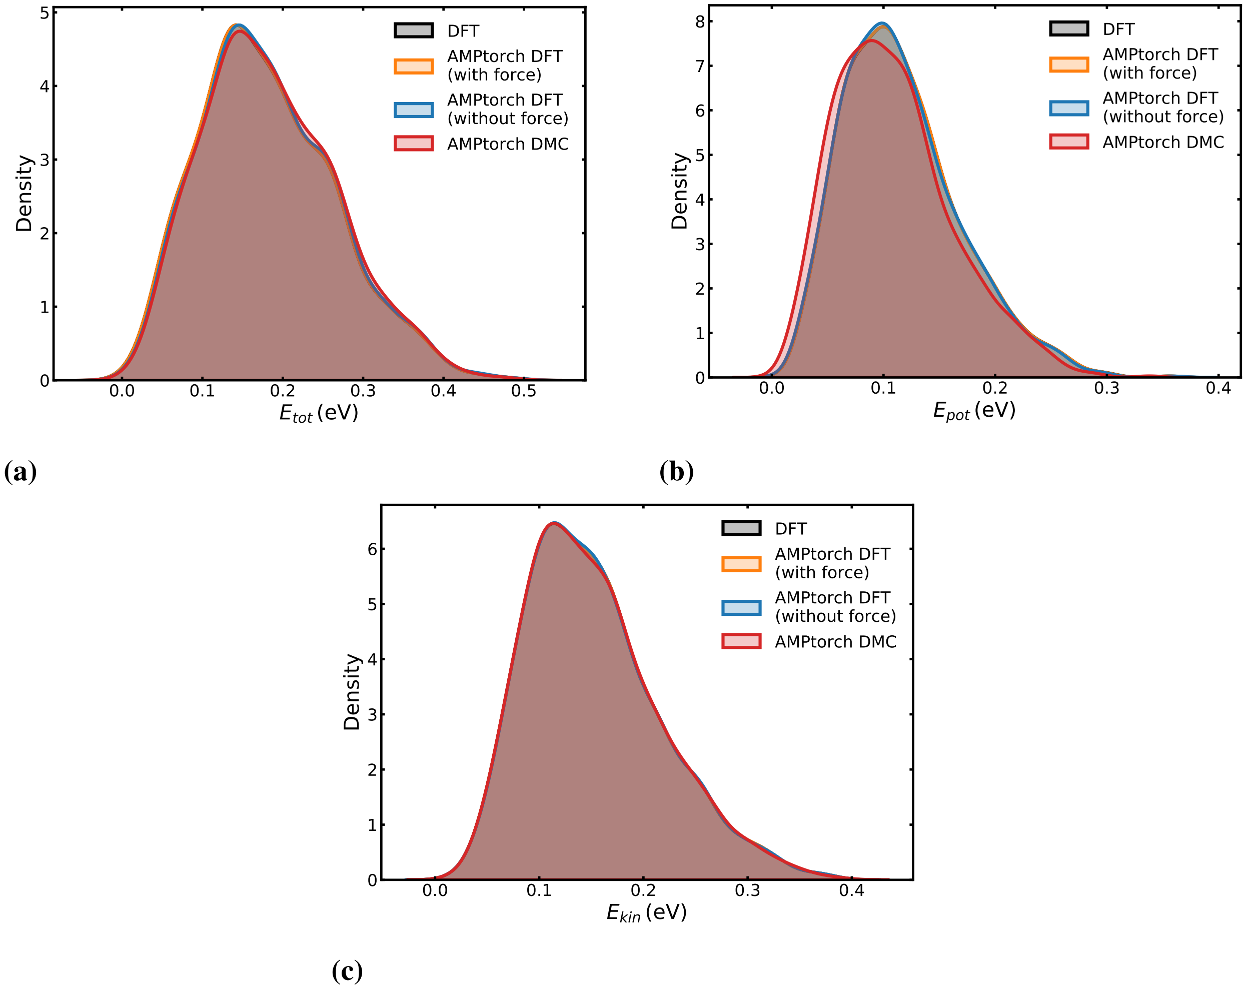


**Figure S33:** Energy distributions from $CH_3Cl$ NVT simulations performed using DFT, the AMPtorch DFT (with forces) model, the AMPtorch DFT (without forces) model, and the AMPtorch DMC model. (a) Density vs. total energy; (b) Density vs. potential energy; and (c) Density vs. kinetic energy.

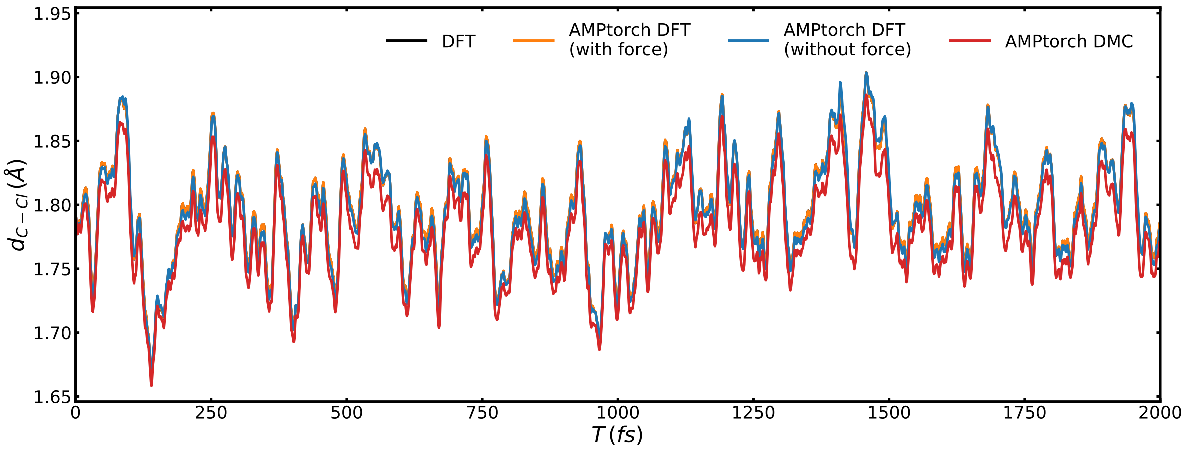


**(a)**

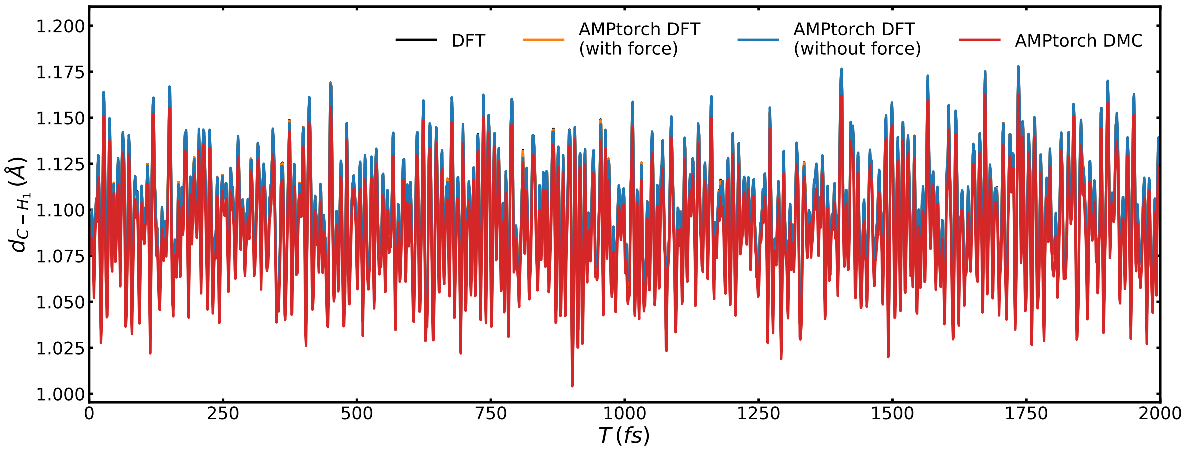


**(b)**

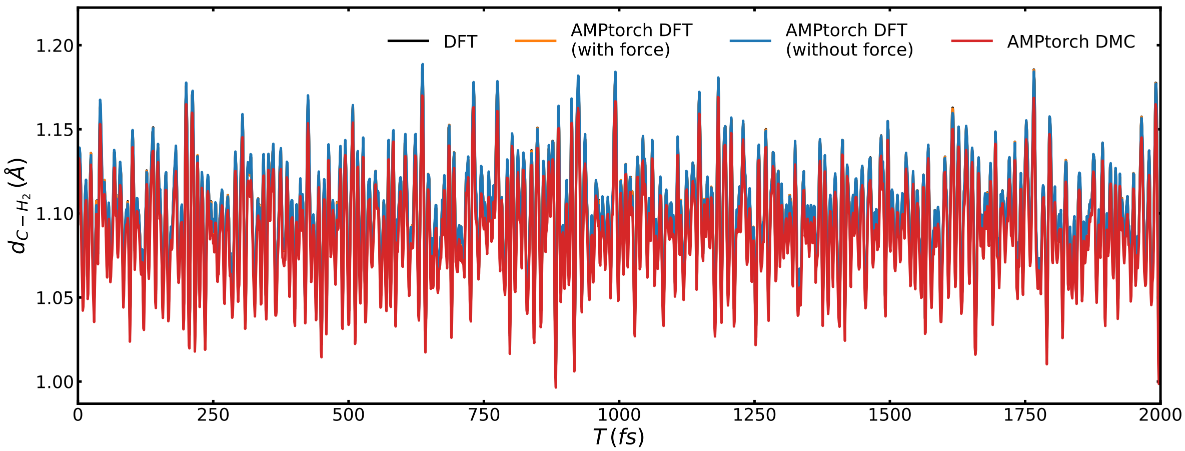


**(c)**

**Figure S34:** Bond distances vs. time from $CH_3Cl$ NVT molecular dynamics simulations.

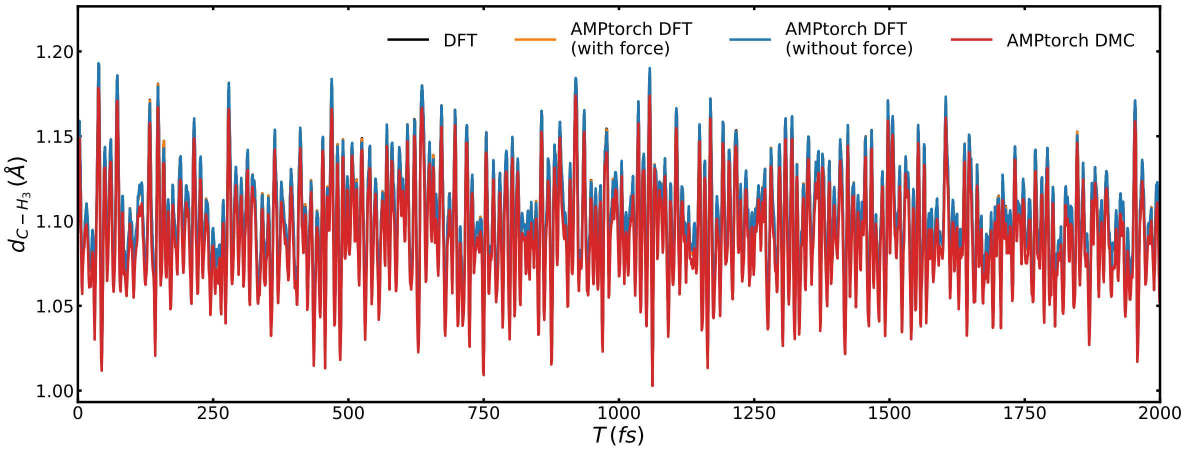


**(a)**

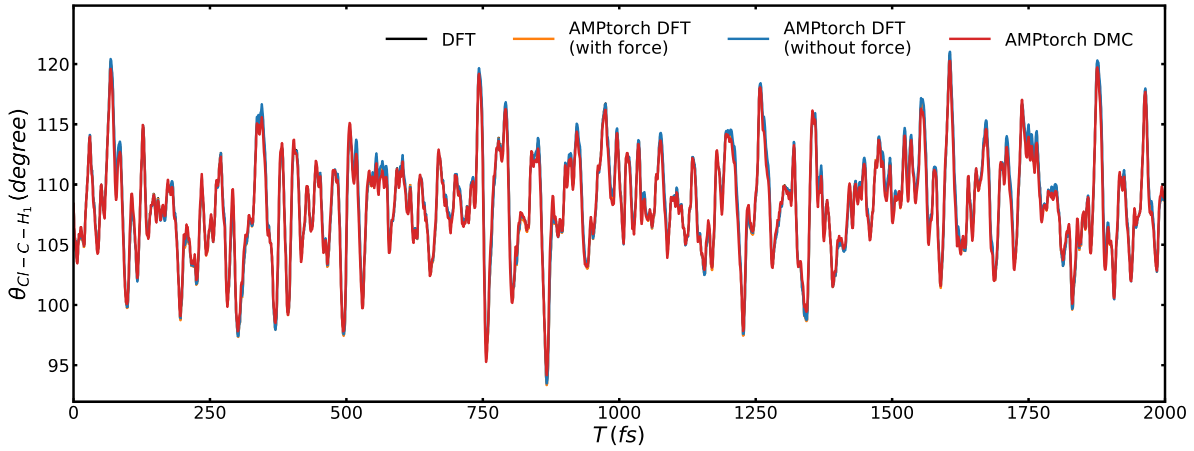


**(b)**

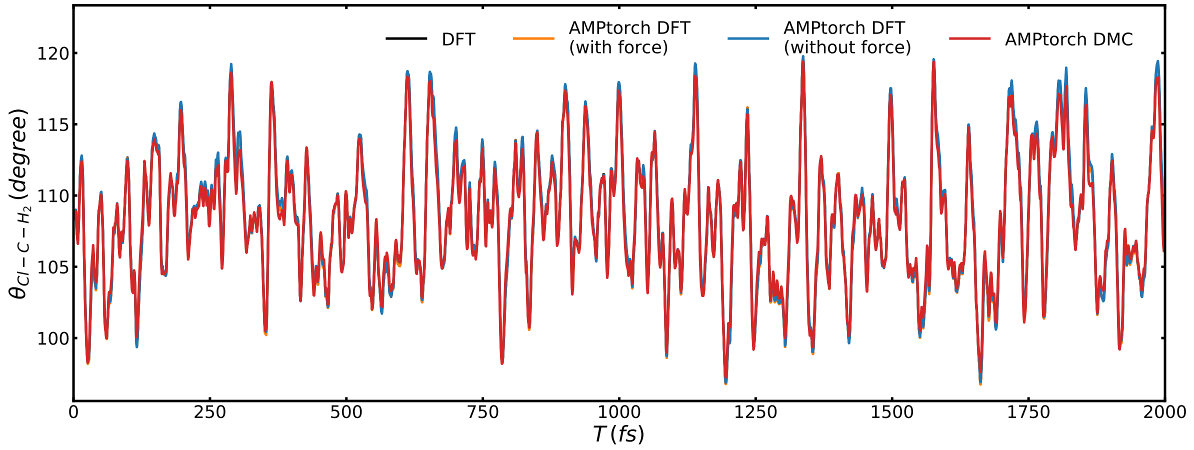


**(c)**

**Figure S35:** Bond distances and angles vs. time from $CH_3Cl$ NVT molecular dynamics simulations.

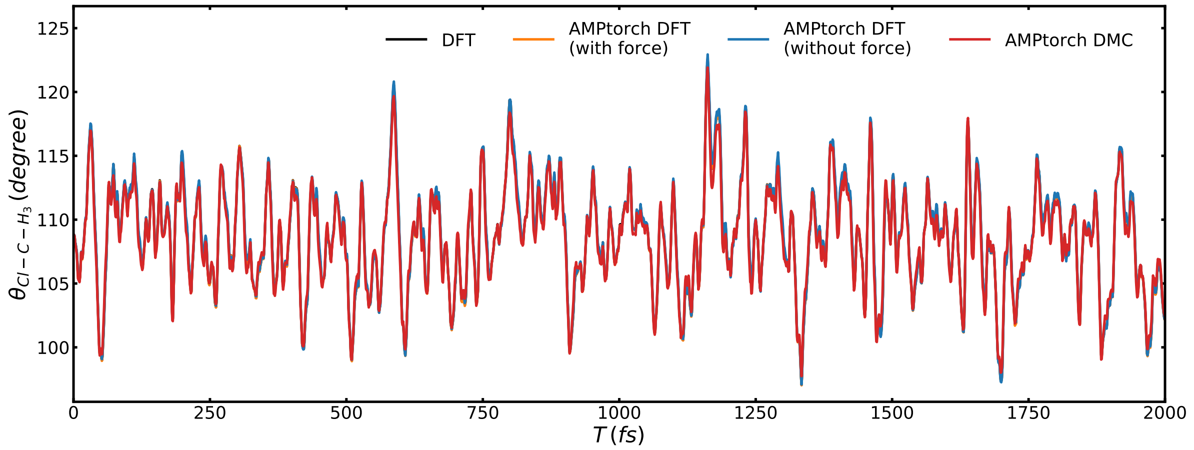


**(a)**

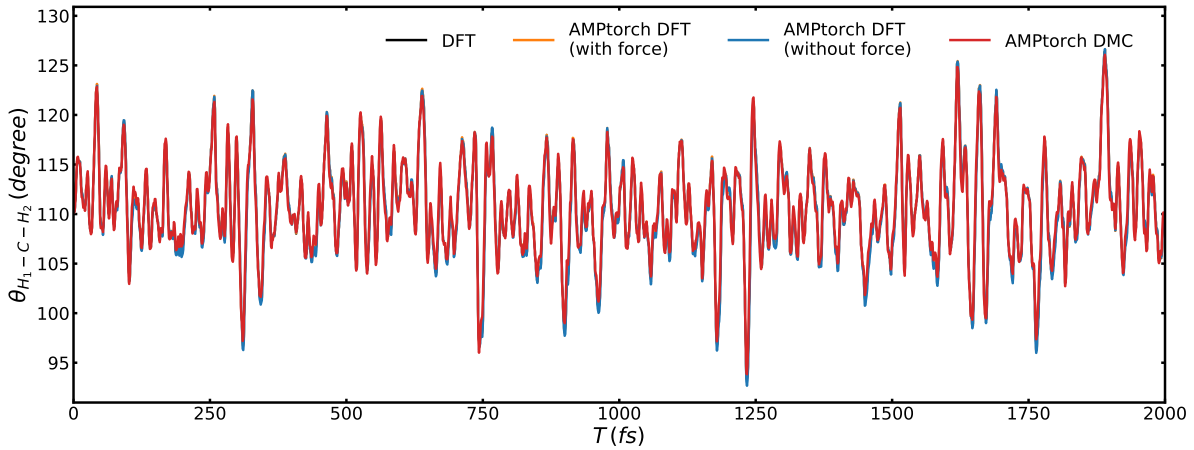


**(b)**

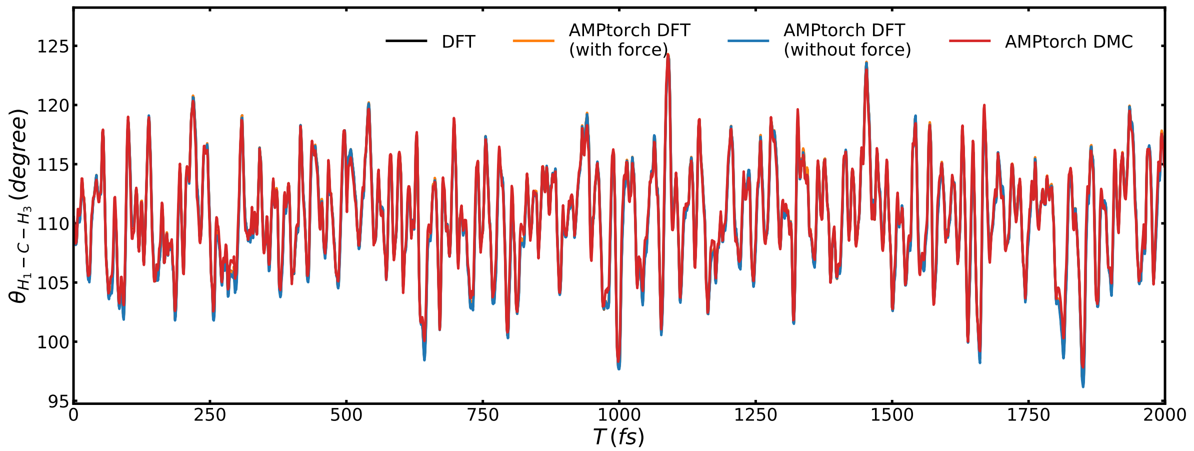


**(c)**

**Figure S36:** Bond angles vs. time from $CH_3Cl$ NVT molecular dynamics simulations.

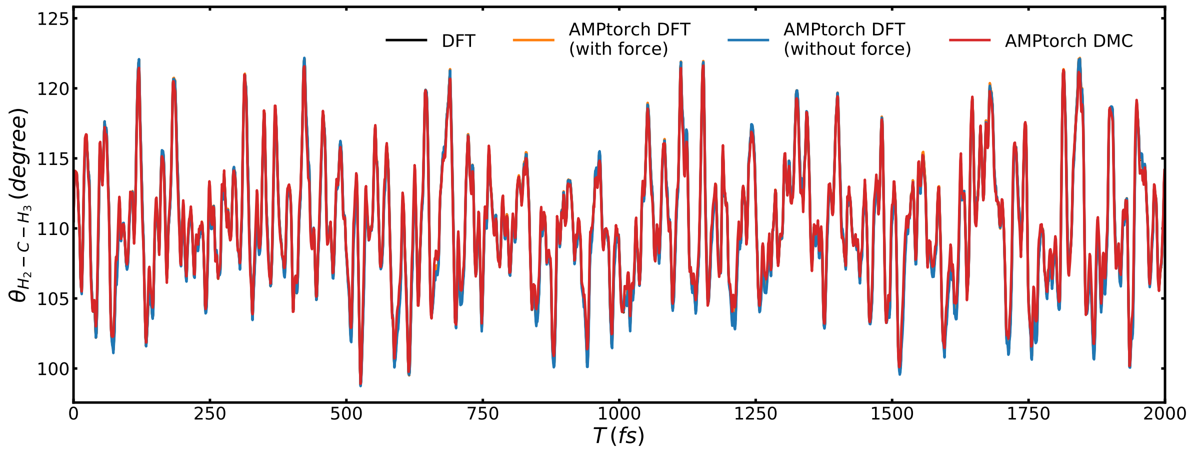


**(a)**

**Figure S37:** Bond angle vs. time from $CH_3Cl$ NVT molecular dynamics simulations.

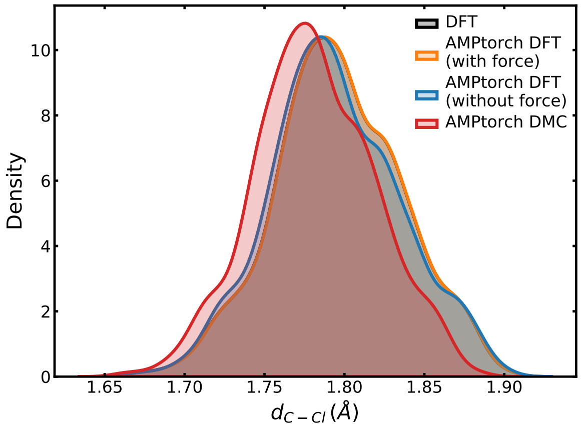


**(a)**

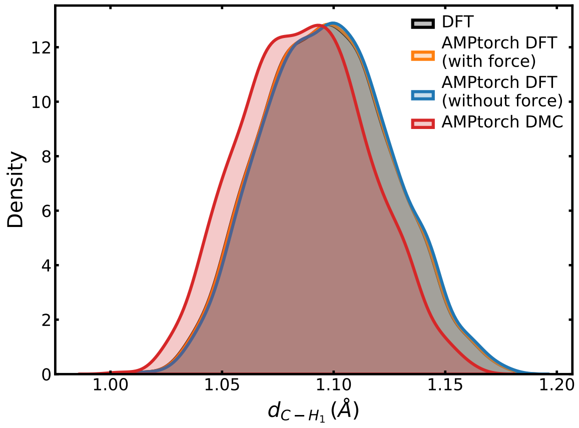


**(b)**

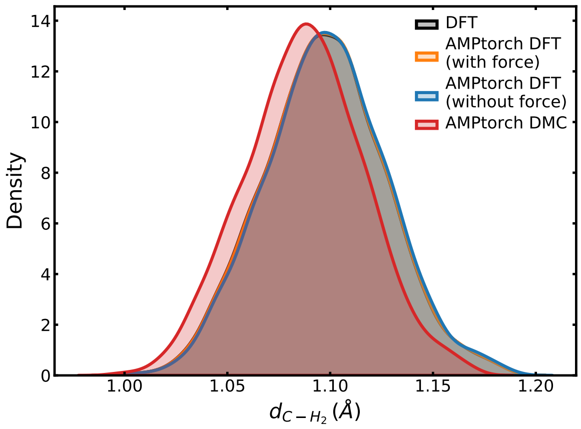


**(c)**

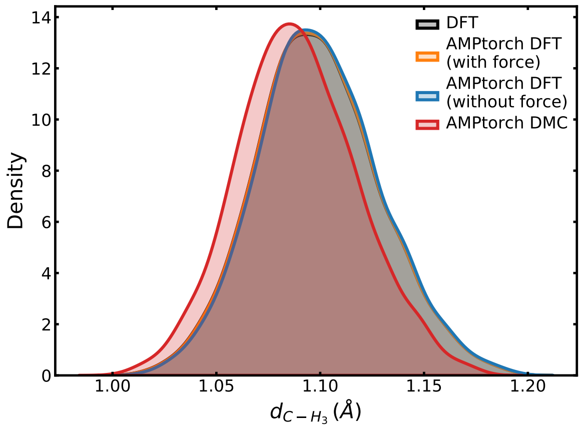


**(d)**

**Figure S38:** Bond distance distributions from $CH_3Cl$ NVT simulations performed using DFT, the AMPtorch DFT (with forces) model, the AMPtorch DFT (without forces) model, and the AMPtorch DMC model.

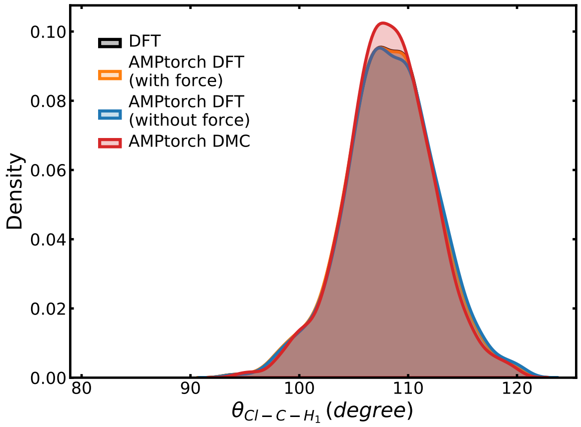


**(a)**

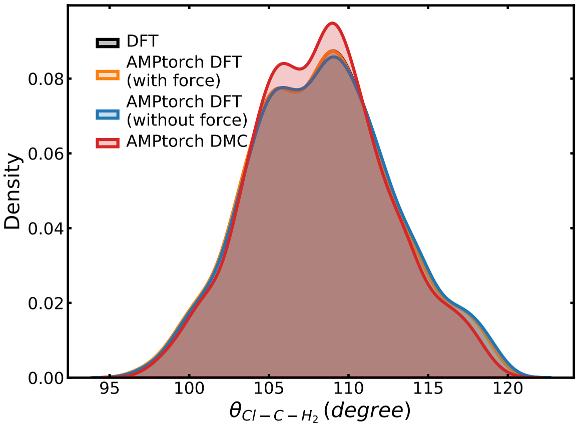


**(b)**

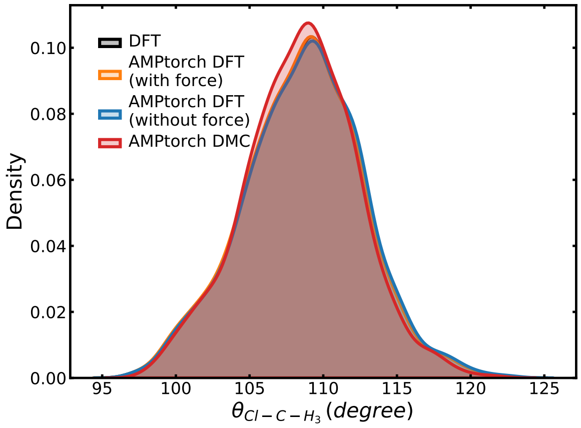


**(c)**

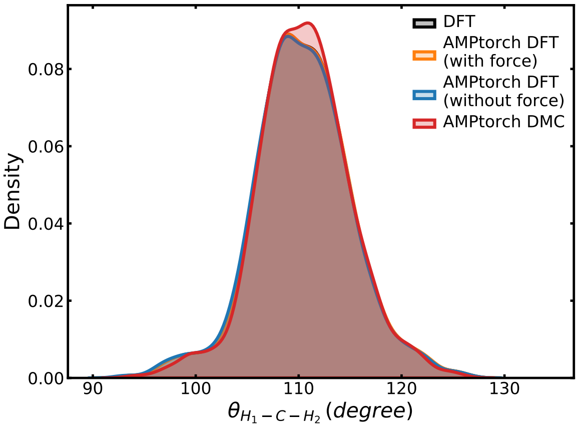


**(d)**

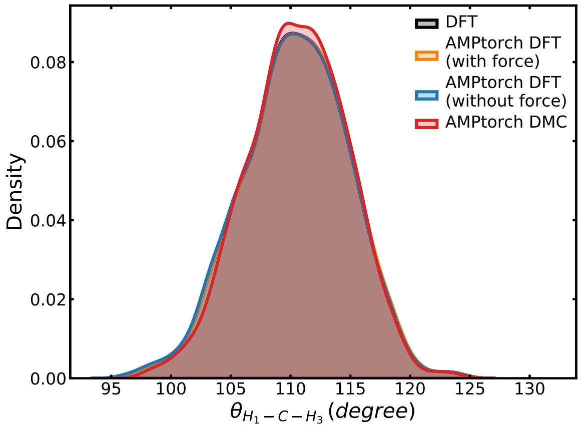


**(e)**

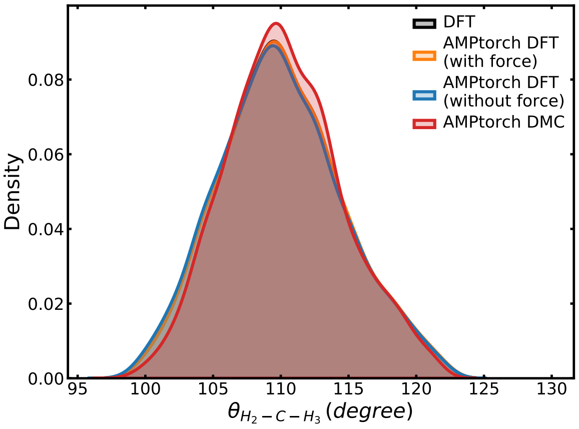


**(f)**

**Figure S39:** Bond angle distributions from $CH_3Cl$ NVT simulations performed using DFT, the AMPtorch DFT (with forces) model, the AMPtorch DFT (without forces) model, and the AMPtorch DMC model.

# Optimization Results

## $H_2O$ Optimization Results

The optimization results for $H_2O$ are shown in Tables S6 - S8.

**Table S6:** Changes in the $d_{O-H_1}$ bond distance during optimization using forces from the different models.

| Step Number | DFT | AMPtorch DFT (with forces) | AMPtorch DFT (without forces) | AMPtorch DMC |
|---|---|---|---|---|
| 0 | 1.3000 | 1.3000 | 1.3000 | 1.3000 |
| 1 | 1.1444 | 1.1355 | 1.1330 | 1.1368 |
| 2 | 0.8218 | 0.8100 | 0.8074 | 0.8151 |
| 3 | 1.0472 | 1.0493 | 1.0496 | 1.0310 |
| 4 | 1.0038 | 1.0118 | 1.0130 | 0.9896 |
| 5 | 0.9438 | 0.9470 | 0.9527 | 0.9437 |
| 6 | 0.9600 | 0.9625 | 0.9606 | 0.9532 |
| 7 | 0.9673 | 0.9711 | 0.9720 | 0.9623 |
| 8 | 0.9677 | 0.9718 | 0.9722 | - |

**Table S7:** Changes in the $d_{O-H_2}$ bond distance during optimization using forces from different models.

| Step Number | DFT | AMPtorch DFT (with force) | AMPtorch DFT (without force) | AMPtorch DMC |
|---|---|---|---|---|
| 0 | 0.9686 | 0.9686 | 0.9686 | 0.9686 |
| 1 | 1.0243 | 1.0315 | 1.0330 | 1.0108 |
| 2 | 1.0422 | 1.0480 | 1.0436 | 1.0198 |
| 3 | 0.9936 | 0.9997 | 0.9992 | 0.9783 |
| 4 | 0.9789 | 0.9859 | 0.9861 | 0.9679 |
| 5 | 0.9620 | 0.9664 | 0.9691 | 0.9611 |
| 6 | 0.9660 | 0.9708 | 0.9718 | 0.9628 |
| 7 | 0.9677 | 0.9726 | 0.9739 | 0.9631 |
| 8 | 0.9674 | 0.9719 | 0.9726 | - |

**Table S8:** Changes in the $\theta_{H_1-O-H_2}$ bond angle during optimization using forces from different models.

| Step Number | DFT | AMPtorch DFT (with force) | AMPtorch DFT (without force) | AMPtorch DMC |
|---|---|---|---|---|
| 0 | 120.00 | 120.00 | 120.00 | 120.00 |
| 1 | 119.70 | 119.96 | 120.02 | 120.30 |
| 2 | 119.40 | 120.28 | 120.81 | 120.60 |
| 3 | 116.49 | 117.19 | 117.59 | 116.90 |
| 4 | 114.10 | 114.69 | 115.43 | 114.08 |
| 5 | 108.36 | 106.91 | 108.95 | 107.47 |
| 6 | 107.41 | 106.12 | 107.04 | 105.33 |
| 7 | 105.16 | 104.00 | 103.04 | 102.83 |
| 8 | 104.31 | 103.52 | 103.56 | - |

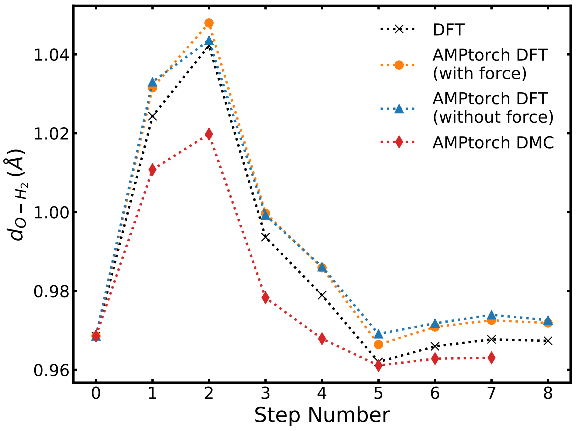


(a)

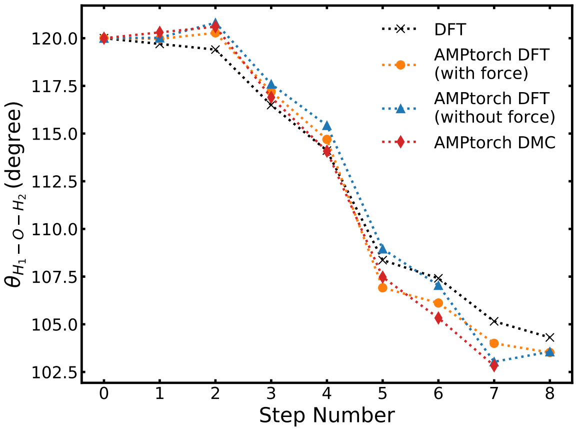


(b)

**Figure S40:** Comparison of the $H_2O$ structural optimization data from simulations using DFT and the trained AMPtorch models: AMPtorch DFT (with forces), AMPtorch DFT (without forces), and AMPtorch DMC. In all cases, the initial $H_2O$ structure is obtained by stretching one O-H bond to 1.3 Å and setting the bond angle to 120°. BFGS method is used for geometry optimization with an fmax value set to 0.05 eV/Å. The optimizations using these models required 8, 10, 16, and 8 iterations, respectively. (a) $d_{O-H_2}$ vs. Step Number (b) $\theta_{H-O-H}$ vs. Step Number

## $CH_3Cl$ Optimization Results

The $CH_3Cl$ optimization results are shown in Tables S9 - S18.

**Table S9:** Changes in the $d_{C-Cl}$ bond distance during optimization using forces from different models.

| Step Number | DFT | AMPtorch DFT (with force) | AMPtorch DFT (without force) | AMPtorch DMC |
|---|---|---|---|---|
| 0 | 1.5238 | 1.5238 | 1.5238 | 1.5238 |
| 1 | 1.8301 | 1.8308 | 1.8243 | 1.8288 |
| 2 | 1.8355 | 1.8352 | 1.8298 | 1.8291 |
| 3 | 1.8295 | 1.8273 | 1.8279 | 1.8036 |
| 4 | 1.8090 | 1.8070 | 1.8091 | 1.7820 |
| 5 | 1.7935 | 1.7929 | 1.7898 | 1.7730 |
| 6 | 1.7938 | 1.7935 | 1.7895 | 1.7750 |
| 7 | 1.7966 | 1.7971 | 1.7903 | 1.7809 |
| 8 | 1.7982 | 1.7989 | 1.7914 | 1.7828 |
| 9 | 1.7985 | 1.7990 | 1.7919 | 1.7824 |
| 10 | 1.7977 | 1.7979 | - | 1.7807 |

**Table S10:** Changes in the $d_{C-H_1}$ bond distance during optimization using forces from different models.

| Step Number | DFT | AMPtorch DFT (with force) | AMPtorch DFT (without force) | AMPtorch DMC |
|---|---|---|---|---|
| 0 | 1.0688 | 1.0688 | 1.0688 | 1.0688 |
| 1 | 1.0637 | 1.0643 | 1.0723 | 1.0585 |
| 2 | 1.0803 | .0808 | 1.0817 | 1.0725 |
| 3 | 1.0903 | 1.0907 | 1.0858 | 1.0838 |
| 4 | 1.0899 | 1.0900 | 1.0852 | 1.0806 |
| 5 | 1.0903 | 1.0901 | 1.0916 | 1.0808 |
| 6 | 1.0919 | 1.0919 | 1.0937 | 1.0824 |
| 7 | 1.0953 | 1.0954 | 1.0968 | 1.0855 |
| 8 | 1.0956 | 1.0958 | 1.0966 | 1.0860 |
| 9 | 1.0947 | 1.0949 | 1.0953 | 1.0854 |
| 10 | 1.0939 | 1.0940 | - | 1.0846 |

**Table S11:** Changes in the $d_{C-H_2}$ bond distance during optimization using forces from different models.

| Step Number | DFT | AMPtorch DFT (with force) | AMPtorch DFT (without force) | AMPtorch DMC |
|---|---|---|---|---|
| 0 | 1.2097 | 1.2097 | 1.2097 | 1.2097 |
| 1 | 1.1201 | 1.1198 | 1.1221 | 1.1139 |
| 2 | 1.1087 | 1.1089 | 1.1113 | 1.1044 |
| 3 | 1.0824 | 1.0834 | 1.0812 | 1.0715 |
| 4 | 1.0800 | 1.0804 | 1.0808 | 1.0740 |
| 5 | 1.0925 | 1.0924 | 1.0937 | 1.0820 |
| 6 | 1.0922 | 1.0922 | 1.0931 | 1.0831 |
| 7 | 1.0937 | 1.0940 | 1.0941 | 1.0856 |
| 8 | 1.0943 | 1.0945 | 1.0947 | 1.0856 |
| 9 | 1.0942 | 1.0943 | 1.0947 | 1.0848 |
| 10 | 1.0938 | 1.0939 | - | 1.0843 |

**Table S12:** Changes in the $d_{C-H_3}$ bond distance during optimization using forces from different models.

| Step Number | DFT | AMPtorch DFT (with force) | AMPtorch DFT (without force) | AMPtorch DMC |
|---|---|---|---|---|
| 0 | 1.2828 | 1.2828 | 1.2828 | 1.2828 |
| 1 | 1.1607 | 1.1606 | 1.1596 | 1.1542 |
| 2 | 1.1272 | 1.1272 | 1.1288 | 1.1167 |
| 3 | 1.0639 | 1.0637 | 1.0612 | 1.0487 |
| 4 | 1.0788 | 1.0790 | 1.0821 | 1.0671 |
| 5 | 1.0921 | 1.0920 | 1.0949 | 1.0821 |
| 6 | 1.0950 | 1.0951 | 1.0967 | 1.0858 |
| 7 | 1.0984 | 1.0986 | 1.0986 | 1.0884 |
| 8 | 1.0969 | 1.0971 | 1.0970 | 1.0869 |
| 9 | 1.0944 | 1.0944 | 1.0950 | 1.0846 |
| 10 | 1.0934 | 1.0934 | - | 1.0838 |

**Table S13:** Changes in the $\theta_{Cl-C-H_1}$ bond angle during optimization using forces from different models.

| Step Number | DFT | AMPtorch DFT (with force) | AMPtorch DFT (without force) | AMPtorch DMC |
|---|---|---|---|---|
| 0 | 102.88 | 102.88 | 102.88 | 102.88 |
| 1 | 95.51 | 95.49 | 95.54 | 95.28 |
| 2 | 96.38 | 96.38 | 96.53 | 96.33 |
| 3 | 101.84 | 101.90 | 102.73 | 102.78 |
| 4 | 105.48 | 105.54 | 105.68 | 106.09 |
| 5 | 107.89 | 107.85 | 108.15 | 107.73 |
| 6 | 107.85 | 107.84 | 108.04 | 107.83 |
| 7 | 107.92 | 107.92 | 108.00 | 108.04 |
| 8 | 108.08 | 108.06 | 108.21 | 108.13 |
| 9 | 108.27 | 108.23 | 108.42 | 108.24 |
| 10 | 108.36 | 108.32 | - | 108.31 |

**Table S14:** Changes in the $\theta_{Cl-C-H_2}$ bond angle during optimization using forces from different models.

| Step Number | DFT | AMPtorch DFT (with force) | AMPtorch DFT (without force) | AMPtorch DMC |
|---|---|---|---|---|
| 0 | 110.93 | 110.93 | 110.93 | 110.93 |
| 1 | 104.09 | 104.09 | 104.37 | 103.91 |
| 2 | 104.34 | 104.36 | 104.55 | 104.12 |
| 3 | 106.11 | 106.19 | 106.26 | 106.39 |
| 4 | 107.70 | 107.79 | 107.58 | 107.73 |
| 5 | 108.42 | 108.46 | 108.47 | 108.27 |
| 6 | 108.45 | 108.48 | 108.51 | 108.30 |
| 7 | 108.37 | 108.36 | 108.48 | 108.25 |
| 8 | 108.30 | 108.28 | 108.45 | 108.22 |
| 9 | 108.28 | 108.25 | 108.44 | 108.23 |
| 10 | 108.32 | 108.29 | - | 108.29 |

**Table S15:** Changes in the $\theta_{Cl-C-H_3}$ bond angle during optimization using forces from different models.

| Step Number | DFT | AMPtorch DFT (with force) | AMPtorch DFT (without force) | AMPtorch DMC |
|---|---|---|---|---|
| 0 | 123.15 | 123.15 | 123.15 | 123.15 |
| 1 | 115.52 | 115.51 | 115.88 | 115.14 |
| 2 | 115.22 | 115.24 | 115.49 | 114.92 |
| 3 | 113.17 | 113.23 | 112.94 | 112.65 |
| 4 | 111.78 | 111.80 | 111.85 | 111.45 |
| 5 | 110.89 | 110.89 | 111.11 | 110.63 |
| 6 | 110.61 | 110.58 | 110.88 | 110.24 |
| 7 | 109.48 | 109.44 | 109.74 | 109.23 |
| 8 | 108.82 | 108.83 | 108.96 | 108.75 |
| 9 | 108.44 | 108.43 | 108.59 | 108.40 |
| 10 | 108.39 | 108.37 | - | 108.33 |

**Table S16:** Changes in the $\theta_{H_1-C-H_2}$ bond angle during optimization using forces from different models.

| Step Number | DFT | AMPtorch DFT (with force) | AMPtorch DFT (without force) | AMPtorch DMC |
|---|---|---|---|---|
| 0 | 99.97 | 99.97 | 99.97 | 99.97 |
| 1 | 105.29 | 105.28 | 104.86 | 105.57 |
| 2 | 105.61 | 105.56 | 105.36 | 105.85 |
| 3 | 108.79 | 108.69 | 109.11 | 109.50 |
| 4 | 110.67 | 110.60 | 110.55 | 111.04 |
| 5 | 111.21 | 111.17 | 110.89 | 111.45 |
| 6 | 111.17 | 111.15 | 110.82 | 111.40 |
| 7 | 110.95 | 111.00 | 110.65 | 111.16 |
| 8 | 110.84 | 110.90 | 110.62 | 110.99 |
| 9 | 110.74 | 110.78 | 110.60 | 110.77 |
| 10 | 110.66 | 110.69 | - | 110.64 |

**Table S17:** Changes in the $\theta_{H_1-C-H_3}$ bond angle during optimization using forces from different models.

| Step Number | DFT | AMPtorch DFT (with force) | AMPtorch DFT (without force) | AMPtorch DMC |
|---|---|---|---|---|
| 0 | 99.68 | 99.68 | 99.68 | 99.68 |
| 1 | 106.08 | 106.08 | 105.77 | 106.37 |
| 2 | 106.72 | 106.71 | 106.59 | 107.15 |
| 3 | 109.41 | 109.38 | 109.98 | 109.63 |
| 4 | 109.76 | 109.72 | 110.03 | 109.83 |
| 5 | 110.09 | 110.07 | 110.16 | 109.95 |
| 6 | 110.03 | 110.03 | 110.05 | 110.00 |
| 7 | 110.22 | 110.26 | 110.08 | 110.35 |
| 8 | 110.45 | 110.49 | 110.27 | 110.54 |
| 9 | 110.61 | 110.65 | 110.41 | 110.66 |
| 10 | 110.61 | 110.64 | - | 110.64 |

**Table S18:** Changes in the $\theta_{H_2-C-H_3}$ bond angle during optimization using forces from different models.

| Step Number | DFT | AMPtorch DFT (with force) | AMPtorch DFT (without force) | AMPtorch DMC |
|---|---|---|---|---|
| 0 | 115.45 | 115.45 | 115.45 | 115.45 |
| 1 | 125.75 | 125.77 | 125.72 | 125.94 |
| 2 | 124.59 | 124.59 | 124.37 | 124.55 |
| 3 | 116.46 | 116.39 | 115.03 | 115.13 |
| 4 | 111.29 | 111.24 | 111.01 | 110.61 |
| 5 | 108.33 | 108.38 | 108.06 | 108.79 |
| 6 | 108.73 | 108.74 | 108.53 | 109.05 |
| 7 | 109.86 | 109.80 | 109.85 | 109.75 |
| 8 | 110.27 | 110.21 | 110.27 | 110.13 |
| 9 | 110.42 | 110.41 | 110.30 | 110.45 |
| 10 | 110.42 | 110.44 | - | 110.54 |

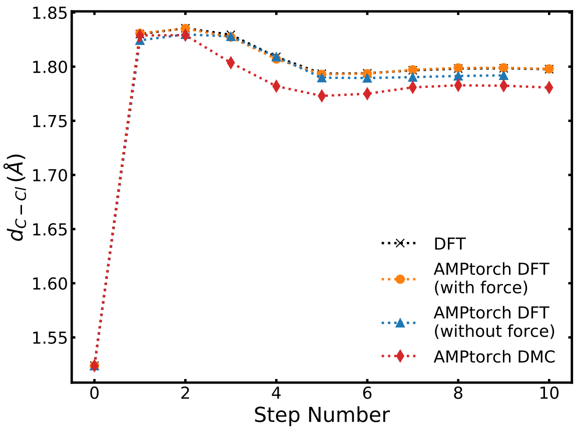


**(a)**

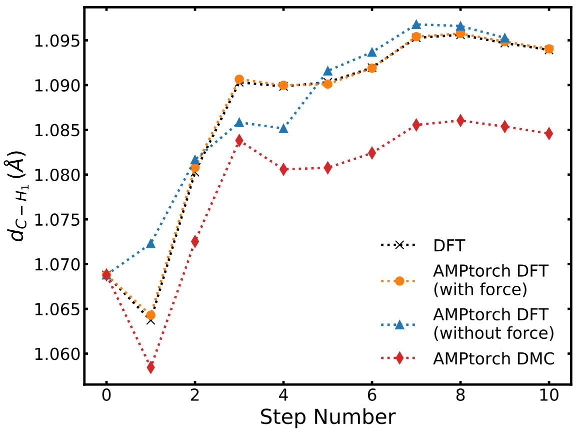


**(b)**

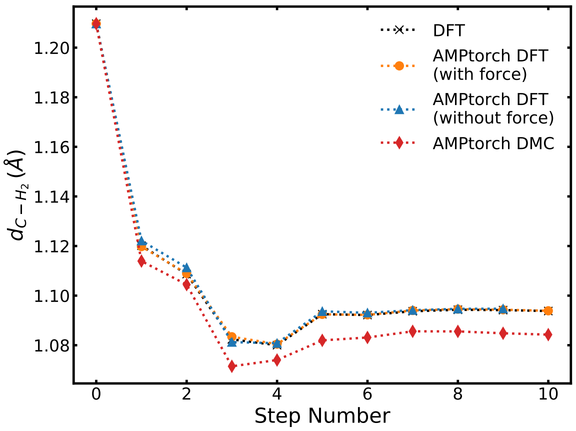


**(c)**

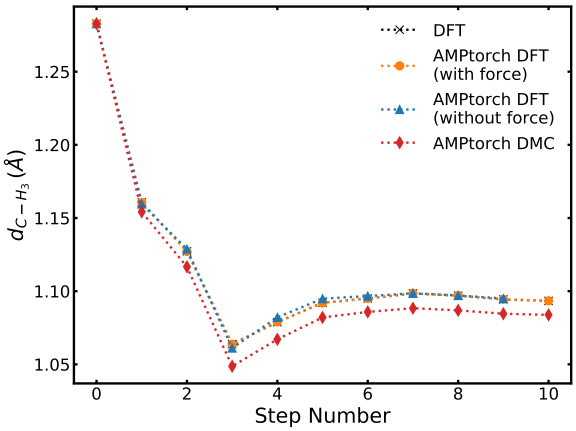


**(d)**

**Figure S41:** Comparison of the $CH_3Cl$ structural optimization of bond lengths from simulations using DFT and the trained AMPtorch models: AMPtorch DFT (with forces), AMPtorch DFT (without forces), and AMPtorch DMC. In all cases, the initial $CH_3Cl$ structure is obtained by randomly displacing the atoms using the *rattle* function, with the standard deviation set to 0.1 Å. The BFGS method is used for geometry optimization with an fmax value set to 0.05 eV/Å. The optimizations using these models required 10, 10, 9, and 10 iterations, respectively. (a) $d_{C-Cl}$ vs. Step Number; (b) $d_{C-H_1}$ vs. Step Number; (c) $d_{C-H_2}$ vs. Step Number; and (d) $d_{C-H_3}$ vs. Step Number.

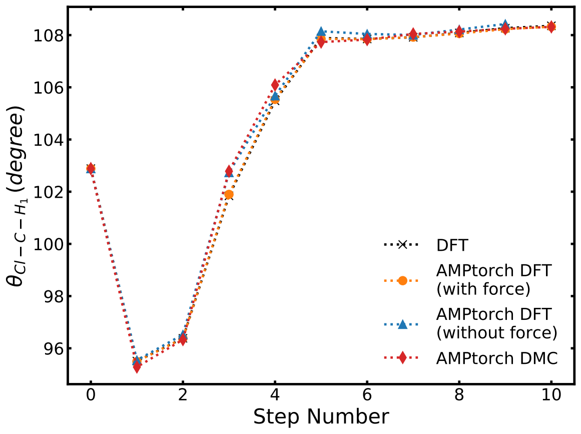


**(a)**

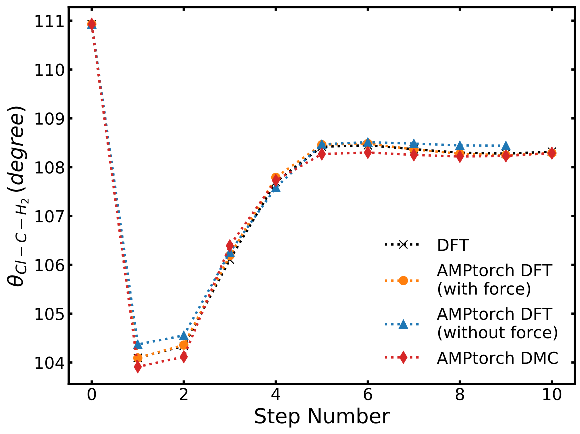


**(b)**

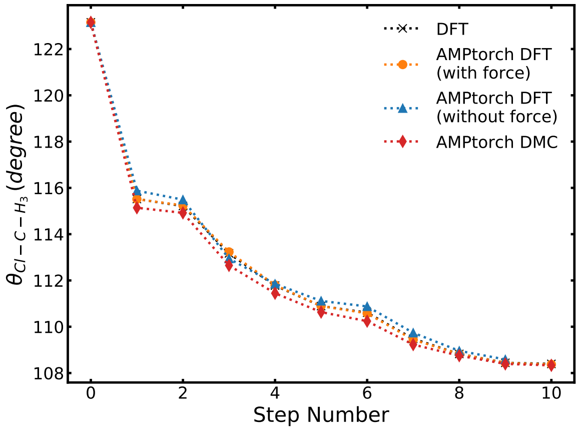


**(c)**

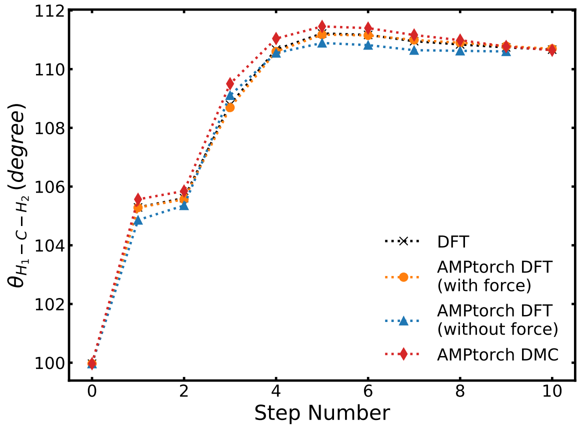


**(d)**

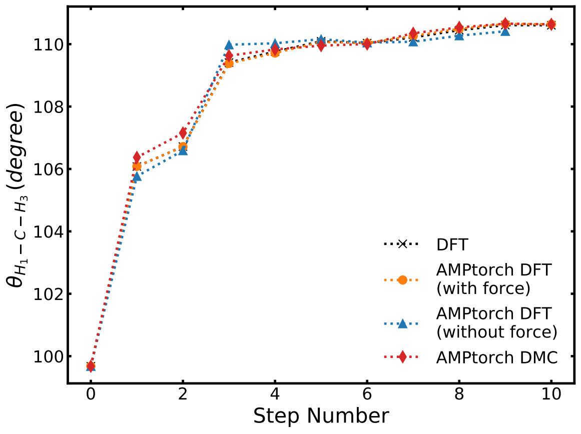


**(e)**

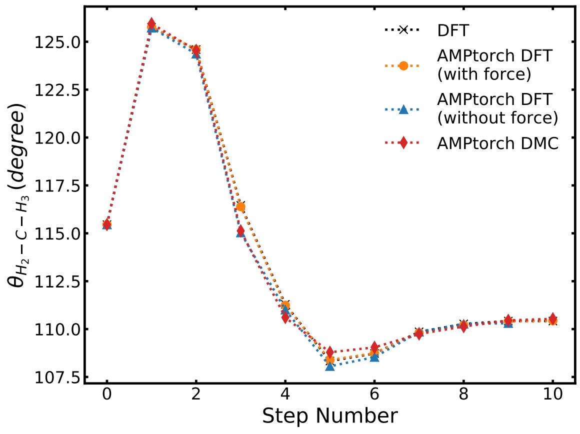


**(f)**

**Figure S42:** Comparison of the $CH_3Cl$ structural optimization of bond angles from simulations using DFT and the trained AMPtorch models: AMPtorch DFT (with forces), AMPtorch DFT (without forces), and AMPtorch DMC. The initial structure is the same as in Figure S41. (a) $\theta_{Cl-C-H_1}$ vs. Step Number; (b) $\theta_{Cl-C-H_2}$ vs. Step Number; (c) $\theta_{Cl-C-H_3}$ vs. Step Number; (d) $\theta_{H_1-C-H_2}$ vs. Step Number; (e) $\theta_{H_1-C-H_3}$ vs. Step Number; and (f) $\theta_{H_2-C-H_3}$ vs. Step Number.

# References


(1) Shuaibi, M.; Sivakumar, S.; Chen, R. Q.; Ulissi, Z. W. Enabling Robust Offline Active Learning for Machine Learning Potentials Using Simple Physics-Based Priors. *Mach. Learn.: Sci. Technol.* **2020**, *2*, 025007.

(2) Owens, A.; Yurchenko, S. N.; Yachmenev, A.; Tennyson, J.; Thiel, W. Accurate Ab Initio Vibrational Energies of Methyl Chloride. *J. Chem. Phys.* **2015**, *142*, 244306.
